# Supplementary material for: ER-Test: Evaluating Explanation Regularization Methods for Language Models
Source: arXiv:2205.12542 source file (2023-02-28)
Supplement: Supplementary file 1 [file 8_appendix_v0.tex]

\section{Appendix} 
\label{sec:appendix}
% \vspace{-0.2cm}

\aaron{Update this}

\subsection{Section 2 Appendix}
\label{sec:app:sec2}

$\mathcal{G}$ first computes raw importance scores $\mathbf{s}_i \in \mathbb{R}^n$, then normalizes $\mathbf{s}_i$ as probabilities $\mathbf{r}_i$ using the sigmoid function.

Broadly, heuristic $\mathcal{G}$'s can either be a gradient-based, that assign importance scores based on gradient changes in $\mathcal{F}$ \cite{sundararajan2017axiomatic, sanyal-ren-2021-discretized, deeplift}, sampling-based, that assign important scores based on the neighbours/context of a given token \cite{occlusion, jin2019towards}, or attention-based, that use the attention-scores or a function of them to assign importance scores. \cite{saliency}.

\subsection{Section 3 Appendix}

\subsubsection{ID Generalization}
\label{sec:app:id}
While \method's main focus is on evaluating OOD generalization, \method also considers ID generalization as a baseline evaluation.
Let $\mathcal{D} = \{\mathcal{X}, \mathcal{Y}\}_{i=1}^{N}$ be a $M$-class text classification dataset, where $\mathcal{X} = \{\mathbf{x}_i\}_{i=1}^{N}$ are the text inputs, $\mathcal{Y} = \{\dot{y}_i\}_{i=1}^{N}$ are the target classes, and $N$ is the number of instances $(\mathbf{x}_i, \dot{y}_i)$ in $\mathcal{D}$.
We call $\mathcal{D}$ the ID dataset.
Assume $\mathcal{D}$ can be partitioned into train set $\mathcal{D}_{\text{train}}$, dev set $\mathcal{D}_{\text{dev}}$, and test set $\mathcal{D}_{\text{test}}$, where $\mathcal{D}_{\text{test}}$ is an ID test set for $\mathcal{D}$.
After using ER to train $\mathcal{F}$ on $\mathcal{D}_{\text{train}}$, we measure $\mathcal{F}$'s task performance on the ID test set $\mathcal{D}_{\text{test}}$.
Note that this is a standard protocol used by existing works to evaluate ER models \cite{zaidan2008modeling, rieger2020interpretations, liu2019incorporating, ross2017right, huang2021exploring, ghaeini2019saliency, kennedy2020contextualizing}

\subsubsection{Contrast Sets}
\label{sec:app:contrast}
Given $\tilde{\mathcal{D}}_{\text{test}}^{(i)}(j)$ (a $j^{th}$ instance belonging to an OOD test set $\tilde{\mathcal{D}}_{\text{test}}^{(i)}$), a perturbation function $\beta_{p}^{(i)}$ is applied to that instance, where $p$ denotes the kind of perturbation taking effect, and it often changes the target label for that instance. For example, $p$ can signify semantic ($\eg$ changing \textit{tall} to \textit{short}), numeral ($\eg$ changing \textit{one dog} to \textit{three dogs}), or  entities ($\eg$ changing \textit{dogs} to \textit{cats}). Each perturbation type is specific to the dataset it is being created for, so that instance labels are changed in a meaningful manner. The resulting set of instances $\mathcal{C^{(i)}} = \beta_{p}^{(i)} (\tilde{\mathcal{D}}_{\text{test}}^{(i)}(j)) \forall j, p$ are termed as a \textit{contrast set} for that dataset. Based on the way they are created, contrast sets are a property of the dataset, and are not created to explicitly challenge $\mathcal{F}$ (unlike adversarial examples \cite{gao2019perturbation}).

\subsubsection{Functional Tests}
\label{sec:app:functional}

\paragraph{Vocabulary Tests}

Vocabulary tests are used to evaluate $\mathcal{F}$'s capability to address changes in the vocabulary of the text, and is particularly diverse w.r.t the parts-of-speech it caters to. For example, certain vocabulary tests evaluate the relationship (taxonomy) between different nouns in a sentence, whereas some swap the modifiers or the verbs present in a sentence in a meaningful manner based on the task at hand, to capture $\mathcal{F}$'s targeted performance towards such changes \cite{ribeiro2020beyond}.
% \aaron{Add citations for this test type.}

\paragraph{Robustness Tests}

Robustness tests evaluate $\mathcal{F}$'s behavior under character-level edits to words in a sentence, keeping the rest of the context same so as to not change the overall prediction. They include testing against typos as well as contractions in words, as well as addition of tokens that are irrelevant for the downstream task (like URLs or gibberish like Twitter handles). \cite{jones-etal-2020-robust, wang-etal-2020-cat}

\paragraph{Logic Tests} 

Testing $\mathcal{F}$'s reasoning capabilities towards logical changes in a sentence is also important to evaluate its reliance on shortcut-patterns. These tests perturb sentences in a logical manner (by adding or removing negations, or purposefully inducing contradictions) that also change the target label in the same manner. \cite{talman2018testing, mccoy-etal-2019-right}

\paragraph{Entity Tests}

For certain tasks, named entities like numbers, locations and proper nouns are not relevant for predicted a target label, and are often a source of gender or demographic biases \cite{mishradembias, gendermehrabi}. Entity tests measure $\mathcal{F}$'s sensitivity towards changes in named entities such that the overall context as well as the task label remains the same~\cite{ribeiro2020beyond}.
% \aaron{Add citations for this test type.}




\begin{figure*}[ht]
    \vspace{-0.5cm}
    \centering
    \includegraphics[width=\linewidth]{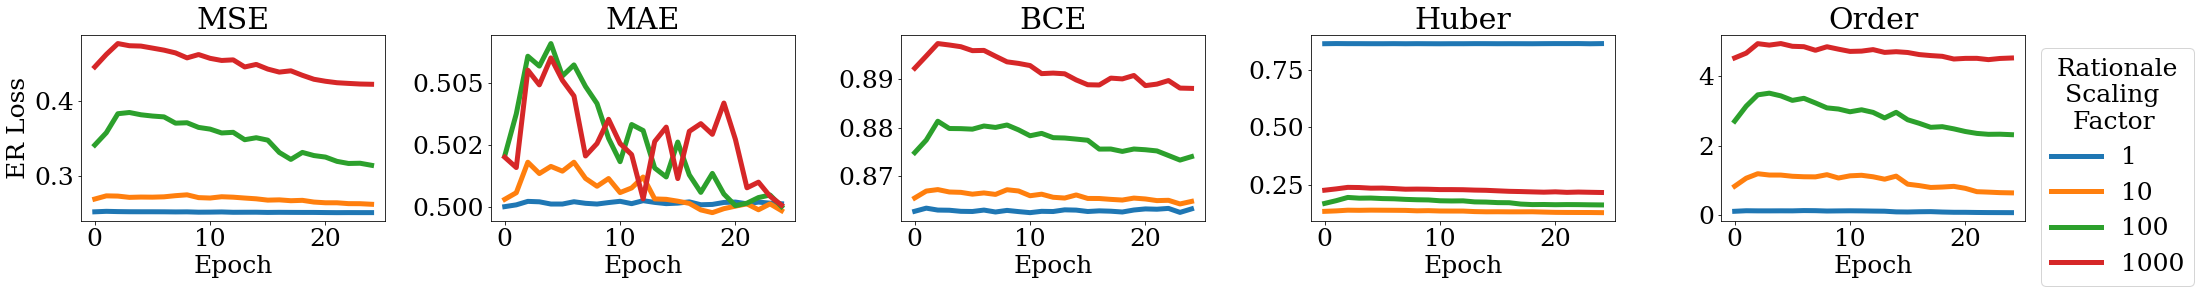}
    \vspace{-0.2cm}
    \caption{\small \textbf{ER Loss Curves (Rationale Scaling Factor).} For rationale extractor, we use IxG}
    \label{fig:exp:int:scale}
\end{figure*}
\subsection{Section 4 Appendix}
\subsubsection{Tasks and Datasets}
\label{sec:app:tasks_datasets}

% \aaron{Add descriptions of how each OOD dataset differs from the ID dataset.}
To evaluate ER models, \method considers a diverse set of sequence and token classification tasks.
For each, task \method provides one ID dataset (annotated with human rationales) and multiple OOD datasets.
Compared to prior works, \method's task/dataset diversity enables more extensive analysis of ER model generalization.

First, we have sentiment analysis, using SST (movie reviews) \cite{socher2013recursive, carton2020evaluating} as the ID dataset.
For OOD datasets, we use Yelp (restaurant reviews) \citep{zhangCharacterlevelConvolutionalNetworks2015}, Amazon (product reviews) \citep{mcauley2013hidden}, and Movies (movie reviews) \cite{zaidan2008modeling, deyoung2019eraser}.
% SST and Movies contain movie reviews, Yelp and Amazon contain restaurant and product reviews, respectively.
Movies' inputs are much longer than the other three datasets'. For contrast set tests, we use an OOD contrast set for sentiment analysis released by the authors of the original paper \cite{gardner2020evaluating}, which are created for the Movies dataset. Furthermore, for functional tests, we use an OOD test suite (flight reviews) from the \texttt{CheckList} \cite{ribeiro2020beyond} which contains both template-based instances to test linguistic capabilities, as well as real-world data (tweets).

Second, we have natural language inference (NLI), using e-SNLI \cite{camburu2018snli, deyoung2019eraser} as the ID dataset.
For the OOD dataset, we use MNLI \cite{williams2017broad}.
e-SNLI contains only image captions, while MNLI contains both written and spoken text, covering various topics, styles, and formality levels. For NLI, we also use an OOD contrast set created for the MNLI dataset \cite{li-etal-2020-linguistically}. Functional tests for NLI are generated from the \texttt{AllenNLP} test suite \cite{Gardner2017AllenNLP} for textual entailment. 

Third, we have named entity recognition (NER), using CoNLL-2003 \cite{sang2003introduction, lin2020triggerner} as the ID dataset.
For the OOD dataset, we use OntoNotes v5.0 \cite{pradhan2013towards}.
CoNLL-2003 contains only Reuters news stories, while OntoNotes v5.0 contains text from newswires, magazines, telephone conversations, websites, and other sources.
\subsubsection{Intrinsic Evaluation of ER}
\label{sec:app:intrinsic_main}
ER in general is sensitive to certain hyperparameters for yielding meaningful training curves and actually attaining alignment between machine and human rationales. Due to a large set of tunable hyperparameters, running all configurations of ER are not feasible. Therefore, we intrinsically evaluate hyperparameter configurations by assessing the loss curves (which model alignment between machine and human rationales) w.r.t different hyperparameters values. We observe that the acceptable band of learning rates for ER is very narrow, and we use $2\mathrm{e}{-5}$ in all of our experiments. Furthermore, we also observe that setting $\lambda_{\text{ER}}=1$ and $\gamma_{\text{ER}}=100$ yields the most drop in the loss curves while training, so we use these hyperparameters for the rest of our experiments. We detail these experiments in Appendix \ref{sec:app:hyperparameters}.
% \xiang{Mention briefly about the motivation for doing intrinsic evaluation before the extrinsic one, and summarize the findings. Point to appendix section for more details.}
\begin{figure}[t!]
    \centering
    \includegraphics[width=\linewidth]{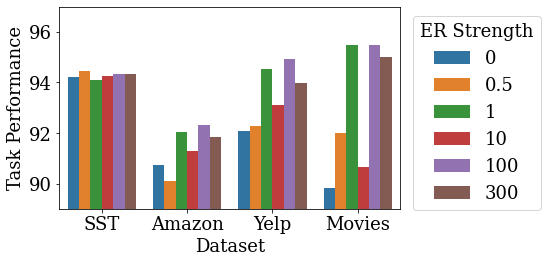}
    \caption{\textbf{ER Strength \versus Task Performance.} For various combinations of sentiment analysis dataset and ER strength, we plot task performance using IxG+MAE.}
    \label{fig:exp:ext:strength}
\end{figure}
\subsubsection{Intrinsic Evaluation: evaluating ER's sensitivity to hyperparameters}
\label{sec:app:hyperparameters}

When using ER to train $\mathcal{F}$, it is important to assess whether ER exhibits expected training behavior, orthogonally to task performance.
If ER improves task performance, this kind of analysis can help us better understand ER's effectiveness.
Conversely, if ER does not improve task performance, such analysis can help us identify the problem.

Let $\gamma_{\text{ER}} > 0$ be the \textit{rationale scaling factor}, used to scale $\mathbf{\hat{s}}_{i}$ prior to sigmoid normalization.
If the magnitudes of the $\mathbf{\hat{s}}_{i}$ scores are lower, then the $\mathbf{\hat{r}}_{i}$ scores will be closer to 0.5 (\ie lower confidence).
However, scaling $\mathbf{\hat{s}}_{i}$ by $\gamma_{\text{ER}} > 1$ will increase the magnitude of $\mathbf{\hat{s}}_{i}$, yielding $\mathbf{\hat{r}}_{i}$ scores closer to 0 or 1 (\ie higher confidence).

Motivated by this, \method's intrinsic evaluation is based on \textit{machine-human rationale alignment}, captured by the ER loss $\mathcal{L_{\text{ER}}} = \Phi(\mathbf{\hat{r}}_{i}, \mathbf{\dot{r}}_{i})$.
When using ER, we should generally expect the ER loss to decrease as $\mathcal{F}$ is trained.
In practice, this may not always be the case, even when ER leads to slightly higher task performance (which is likely a mirage caused by lucky random seeds)!
That is, by definition, non-decreasing ER loss signals ineffective ER usage, since the machine rationales are not becoming more similar to the human rationales.
This can stem from a number of issues: \eg poor choice of ER criteria $\Phi$, improper ER strength $\lambda_{\text{ER}}$, improper rationale scaling factor $\gamma_{\text{ER}}$, noisy human rationale $\mathbf{\dot{r}}_{i}$, insufficient $\mathcal{F}$ capacity.
Thus, we measure machine-human rationale alignment as the first step in diagnosing such issues.
Let \textit{ER loss curve} denote a chart which plots $\mathcal{L_{\text{ER}}}$ \versus the number of train epochs.
For each combination of ER criteria $\Phi$ and some training configuration, we plot ER loss curves for the training set.
% \aaron{Do we plot both train and dev ER loss?}
Each component of our intrinsic evaluation varies a different hyperparameter in the training configuration: (A) ER strength $\lambda_{\text{ER}}$; (B) rationale scaling factor $\gamma_{\text{ER}}$; and (C) learning rate $\alpha$.
% To compare different $\Phi$ for a given training setting, we display all loss curves for the same dataset split (\ie train or dev) on the same plot.
% \aaron{Do we normalize the loss curves? Is this feasible? Does it make sense?}
% (\eg w.r.t. rationale extractor $\mathcal{G}$, ER strength $\lambda_{\text{ER}}$, scaling factor for $\mathbf{\hat{r}}_{i}$)
In contrast, prior works do not explore the relationship between $\mathcal{L_{\text{ER}}}$ and these training variables \cite{huang2021exploring, ghaeini2019saliency}.

% \subsection{Intrinsic Evaluation}
For intrinsic evaluation, we use ER strength $\lambda_{\text{ER}}=1$, rationale scaling factor $\gamma_{\text{ER}}=1$, and learning rate $\alpha=2\mathrm{e}{-5}$, unless otherwise specified.
As a proof of concept, we focus on SST here, but plan to add other datasets in future work.

\subsubsection{Misc. Details}
All models are trained on GeForce GTX 1080 Ti and Quadro RTX 6000 GPUs. All implementations are done using the HuggingFace API \cite{huggingface}. 

\subsubsection{ER Strength}
\label{sec:app:int:strength}
Fig. \ref{fig:exp:int:strength} displays the ER loss curves for different ER strengths $\lambda_{\text{ER}}=[0.5, 1, 10, 100, 300]$, on SST using MAE.
Among the $\lambda_{\text{ER}}$ values, we see that $\lambda_{\text{ER}}=1$ yields ER loss curves with the greatest decrease (Table \ref{tab:exp:int:strength}), signaling good ER optimization.
% We empirically validate the use of this $\lambda_{\text{ER}}=1$ prior in Table \ref{tab:exp:use:hparam}.
% See \textsection \aaron{insert appendix section} for results.
% \aaron{Need to reference table for more concrete conclusions.}

% \subsubsection{ER Strength}

\subsubsection{Rationale Scaling Factor}
\label{sec:app:int:scale}
Fig. \ref{fig:exp:int:scale} displays the ER loss curves for different rationale scale factors $\gamma_{\text{ER}}=[1, 10, 100, 1000]$, on SST.
Among the four $\gamma_{\text{ER}}$ values, we see that $\gamma_{\text{ER}}=100$ yields ER loss curves with the greatest decrease (Table \ref{tab:exp:int:scale}), signaling good ER optimization.
Meanwhile, although ER works use $\gamma_{\text{ER}}=1$ by default, we see that $\gamma_{\text{ER}}=1$ yields nearly flat ER loss curves for all five $\Phi$ choices.
This suggests poor ER optimization.
Based on these results, we fix $\gamma_{\text{ER}}=100$ for all experiments (\textsection \ref{sec:exp}), thus greatly reducing the hyperparameter search space.
% \aaron{reference Table \ref{tab:exp:int:strength}}
% \aaron{Need to reference table for more concrete conclusions.}
% In \textsection \ref{sec:exp:use:hparam}, we empirically validate the usage of this $\gamma_{\text{ER}}=100$ prior.
% See \textsection \aaron{insert appendix section} for results on other datasets. 
\begin{figure*}
    \centering
    \includegraphics[width=\linewidth]{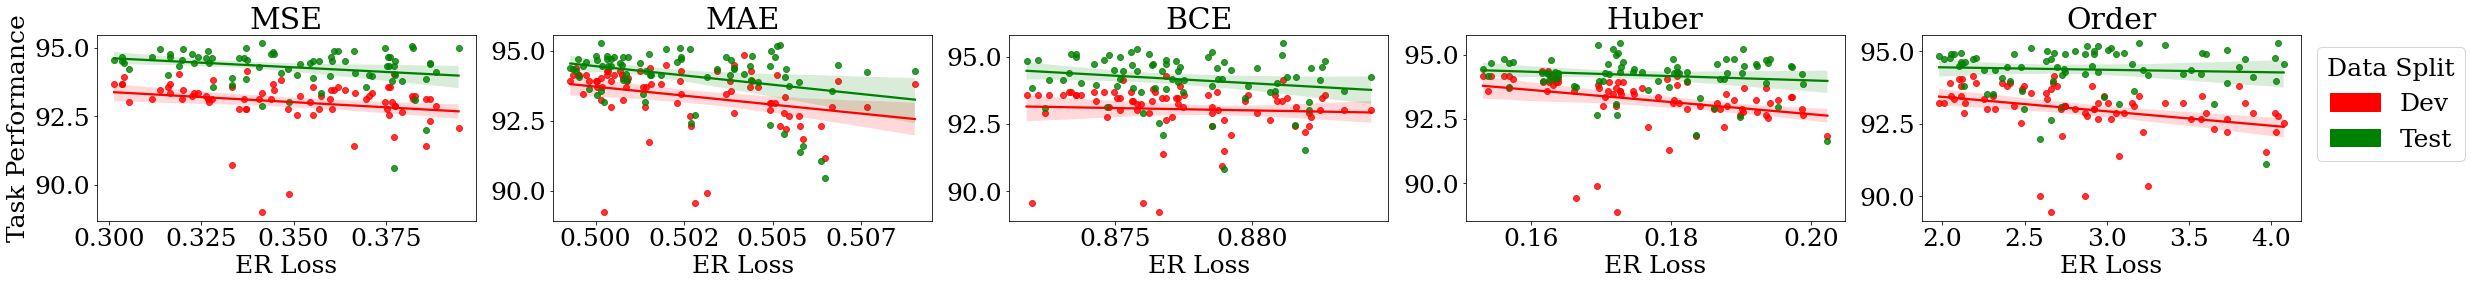}
    \caption{\small \textbf{Task Performance vs. ER Loss}. Here we use IxG as rationale extractor}
    \label{fig:exp:ext:loss}
\end{figure*}
\subsubsection{Learning Rate}
\label{sec:app:int:lr}
Here, we obtain similar conclusions, with $\alpha=2\mathrm{e}{-5}$ yielding the best ER loss curves. Fig. \ref{fig:exp:int:lr} displays the ER loss curves for different learning rates $\alpha=[2\mathrm{e}{-6}, 2\mathrm{e}{-5}, 2\mathrm{e}{-4}]$.
Among the three learning rates, we see that $\alpha=2\mathrm{e}{-5}$ yields the most steadily decreasing ER loss curves.
\begin{figure*}
    \centering
    \includegraphics[width=\linewidth]{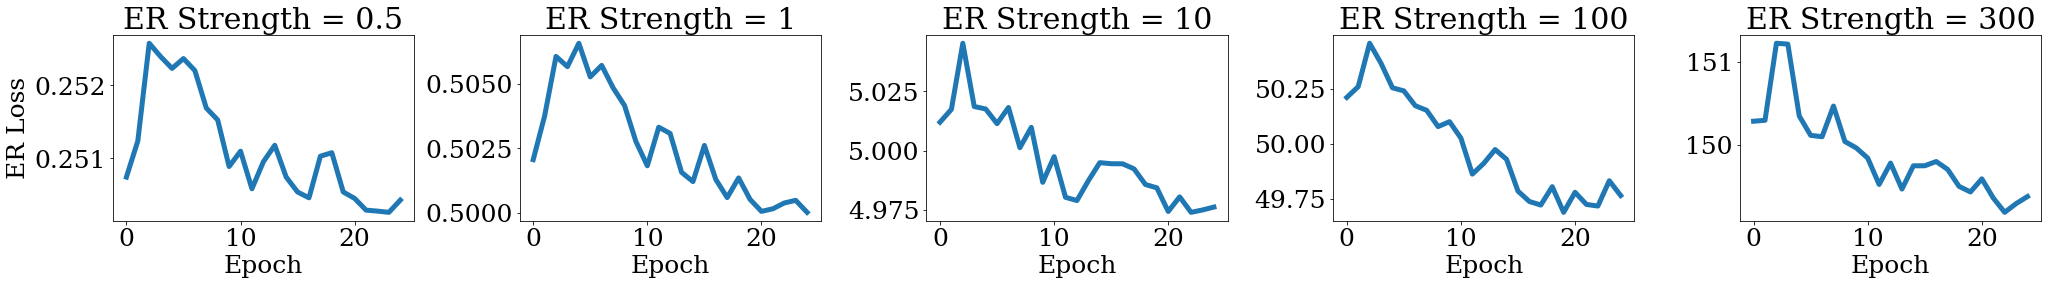}
    \caption{\small \textbf{ER Loss Curves (ER Strength).} Here, we use the MAE criterion and IxG as rationale extractor}
    \label{fig:exp:int:strength}
\end{figure*}




\begin{figure*}
    \centering
    \includegraphics[width=\linewidth]{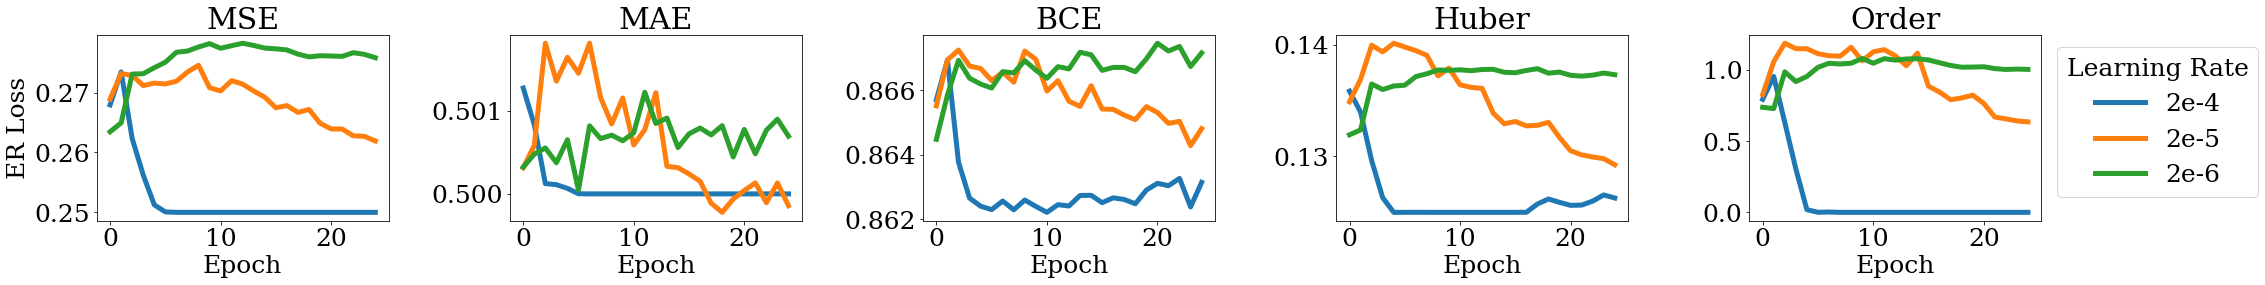}
    \caption{\small \textbf{ER Loss Curves (Learning Rate)}. Here we use IxG as rationale extractor }
    \label{fig:exp:int:lr}
\end{figure*}

\subsubsection{ER performance with different hyperparameters}
\label{sec:app:er_perf}
\begin{table}[t!]
\centering
\scalebox{0.7}{
\begin{tabular}{cccccc}
\toprule
 & \multicolumn{5}{c}{\textbf{ER Strength}} \\
 \cmidrule(lr){2-6}

\textbf{ER criteria} & 0.5 & 1 & 10 & 100 & 300 \\

\midrule

IxG+MSE & 0.91 & \textbf{1.52} & 1.41 & 1.29 & 1.35 \\ 
IxG+MAE & 1.89 & \textbf{2.01} & 1.72 & 1.80 & 1.74 \\ 
IxG+BCE & 1.99 & \textbf{2.17} & 1.65 & 1.65 & 1.75 \\ 
IxG+Huber & 1.85 & 2.09 & 2.24 & 2.27 & \textbf{2.40} \\ 
IxG+Order & 2.15 & 2.40 & 1.60 & \textbf{2.53} & 1.89 \\ 

\bottomrule

\end{tabular}}
\caption{\textbf{Relative Decrease in ER Loss.} For various ER strengths, we report the percentage decrease in ER train loss (on SST), from max point to min point.}
\label{tab:exp:int:strength}
\end{table}
\begin{table}[]
\centering
\scalebox{0.65}{
\begin{tabular}{ccccc}
\toprule
 & \multicolumn{4}{c}{\textbf{Rationale Scaling Factor}} \\
 \cmidrule(lr){2-5}

\textbf{ER criteria} & 1 & 10 & 100 & 1000 \\

\midrule

IxG+MSE & 0.69 & 4.60 & \textbf{18.35} & 11.41 \\
% MAE & 0.91 & \textbf{1.52} & 1.41 & 1.29 & 1.35 & 0.04 & 0.40 & \textbf{1.29} & 1.17 \\ 
IxG+MAE & 0.04 & 0.40 & \textbf{1.29} & 1.17 \\ 
IxG+BCE & 0.10 & 0.34 & 0.90 & \textbf{1.03}\\ 
IxG+Huber & 0.10 & 7.75 & \textbf{16.67} & 9.30 \\ 
IxG+Order & 7.21 & 9.38 & \textbf{47.97} & \textbf{1.89}\\ 

\bottomrule

\end{tabular}}
\caption{\textbf{Relative Decrease in ER Loss.} For various ER rationale scaling factors, we report the percentage decrease in ER train loss (on SST), from max point to min point.}
\label{tab:exp:int:scale}
\end{table}

\paragraph{ER Strength \versus Task Performance}
To measure ER's impact on task performance, we plot $\mathcal{F}$'s task performance as a function of ER strength $\lambda_{\text{ER}}$. 
This is conducted for ID test sets.\\
For each sentiment analysis dataset, Fig. \ref{fig:exp:ext:strength} shows task performance for ER strengths $\lambda_{\text{ER}}=[0, 0.5, 1, 10, 100, 300]$, using MAE.
Note that $\lambda_{\text{ER}}=0$ is equivalent to training the LM without ER (\ie None in Table \ref{tab:exp:rq1:unseen}).
For the ID dataset (SST), we see that all ER strengths yield very similar task performance, suggesting that ER has little effect on ID task performance.
However, for the OOD datasets (Amazon, Yelp, Movies), task performance generally increases as $\lambda_{\text{ER}}$ increases, showing ER's positive impact on LM generalization.
Overall, based on OOD task performance, we find that $\lambda_{\text{ER}}=[1, 100]$ are the best ER strengths.
This aligns with the results of \textsection \ref{sec:app:int:strength}. 
\begin{table}[]
\centering
\scalebox{0.7}{
\begin{tabular}{ccccc}
\toprule
 & \multicolumn{2}{c}{\textbf{Dev}} & \multicolumn{2}{c}{\textbf{Test}} \\
 \cmidrule(lr){2-3} \cmidrule(lr){4-5}
\textbf{ER criteria} & \multicolumn{1}{c}{Slope ($\downarrow$)} & $R^{2}$ ($\uparrow$) & \multicolumn{1}{c}{Slope ($\downarrow$)} & $R^{2}$ ($\uparrow$) \\ 

\midrule

IxG+MSE & \multicolumn{1}{c}{-7.48} & 0.050 & \multicolumn{1}{c}{-6.75} & 0.059 \\
IxG+MAE & \multicolumn{1}{c}{\textbf{-128.60}} & 0.083 & \multicolumn{1}{c}{\textbf{-133.03}} & \textbf{0.110} \\ 
IxG+BCE & \multicolumn{1}{c}{-17.48} & 0.003 & \multicolumn{1}{c}{-56.30} & 0.040\\ 
IxG+Huber & \multicolumn{1}{c}{-23.59} & 0.091 & \multicolumn{1}{c}{-8.40} & 0.022 \\ 
IxG+Order & \multicolumn{1}{c}{-0.49} & \textbf{0.101} & \multicolumn{1}{c}{-0.085} & 0.004 \\ \bottomrule
\end{tabular}}
\caption{\small \textbf{ER Loss \versus Task Performance.} We summarize the line plots in Fig. \ref{fig:exp:ext:loss} (ER Loss \versus Task Performance), using slope and $R^2$ score (\textsection \ref{sec:app:er_perf}). Ideally, Fig. \ref{fig:exp:ext:loss}'s lines would have \textit{low slope} and \textit{high $R^2$}, indicating that ER helps improve task performance. We see that MAE yields the best ER results.}
\label{tab:exp:ext:loss}
\end{table}
% \begin{table*}[t]
\begin{table*}[]
% \vspace{-0.2cm}
\centering
\scalebox{0.67}{
\begin{tabular}{cccccc}
    \toprule
    \multirow{4}{*}{\textbf{ER criteria}} & \multicolumn{4}{c}{\textbf{Sentiment Analysis (Out-of-Domain)}} \\
    \cmidrule(lr){2-5}
    & Amazon & Yelp & Movies & Mean \\
    
    \midrule
    
    {None} & 90.72~($\pm$1.36) & 92.07~($\pm$2.66) & 89.83~($\pm$6.79) & 90.87~($\pm$ 3.60) \\
    
    \midrule
    
    {IxG+MAE ($\lambda_{\text{ER}}=0.5$)} & 90.12~($\pm$2.98) & 92.27~($\pm$3.29) & 92.00~($\pm$5.68) & 91.46~($\pm$0.91) \\
    {\cellcolor{lblue} IxG+MAE ($\lambda_{\text{ER}}=1$)} & \cellcolor{lblue} 92.02~($\pm$0.25) & \cellcolor{lblue} 94.55~($\pm$0.30) & \cellcolor{lblue} 95.50~($\pm$1.32) & \cellcolor{lblue} 94.02~($\pm$2.15) \\
    {IxG+MAE ($\lambda_{\text{ER}}=10$)} & 91.27~($\pm$0.28) & 93.10~($\pm$1.08) & 90.67~($\pm$3.79) & 91.68~($\pm$1.06) \\
    {IxG+MAE ($\lambda_{\text{ER}}=100$)} & \textbf{92.33~($\pm$0.28)} & \textbf{94.92~($\pm$0.56)} & \textbf{95.50~($\pm$0.50)} & \textbf{94.25~($\pm$1.89)} \\
    {IxG+MAE ($\lambda_{\text{ER}}=300$)} & 91.83~($\pm$0.42) & 93.97~($\pm$1.28) & 95.00~($\pm$0.50) & 93.60~($\pm$1.74) \\
    
    \midrule
    
    {IxG+MAE ($\gamma_{\text{ER}}=1$)} & 90.63~($\pm$1.88) & 92.32~($\pm$2.23) & 88.67~($\pm$4.25) & 90.54~($\pm$2.22) \\
    {IxG+MAE ($\gamma_{\text{ER}}=10$)} & \textbf{92.30~($\pm$1.21)} & 93.01~($\pm$2.14) & \textbf{96.83~($\pm$1.04)} & \textbf{94.07~($\pm$3.89)} \\
    {\cellcolor{lblue} IxG+MAE ($\gamma_{\text{ER}}=100$)} & \cellcolor{lblue} 92.02~($\pm$0.25) & \cellcolor{lblue} \textbf{94.55~($\pm$0.30)} & \cellcolor{lblue} 95.50~($\pm$1.32) & \cellcolor{lblue} 94.02~($\pm$2.15) \\
    {IxG+MAE ($\gamma_{\text{ER}}=1000$)} & 90.47~($\pm$2.06) & 92.80~($\pm$2.90) & 92.67~($\pm$6.25) & 91.98~($\pm$1.14) \\
    
    \midrule
    
    {IxG+MAE ($\alpha=2\mathrm{e}{-4}$)} & 89.35~($\pm$2.85) & 91.23~($\pm$2.84) & 93.00~($\pm$2.65) & 91.19~($\pm$2.22) \\
    {\cellcolor{lblue} IxG+MAE ($\alpha=2\mathrm{e}{-5}$)} & \cellcolor{lblue} \textbf{92.02~($\pm$0.25)} & \cellcolor{lblue} \textbf{94.55~($\pm$0.30)} & \cellcolor{lblue} \textbf{95.50~($\pm$1.32)} & \cellcolor{lblue} \textbf{94.02~($\pm$2.15)} \\
    {IxG+MAE ($\alpha=2\mathrm{e}{-6}$)} & 88.60~($\pm$1.60) & 83.27~($\pm$6.49) & 81.17~($\pm$6.93) & 84.34~($\pm$9.70) \\
    
    
    \bottomrule 
\end{tabular}
}
% \vspace{0.3cm}
\caption{\small \textbf{Task Performance \versus \{ER Strength ($\lambda_{\text{ER}}$), Rationale Scaling Factor ($\gamma_{\text{ER}}$)\}.} Higher values are better.}
\label{tab:exp:use:hparam}
% \vspace{-0.3cm}
% \end{table*}
\end{table*}

\paragraph{ER Loss \versus Task Performance}
To measure ER's impact on task performance, we plot $\mathcal{F}$'s task performance as a function of ER loss $\mathcal{L}_{\text{ER}}$.
This is conducted for both ID and OOD test sets.\\
Fig. \ref{fig:exp:ext:loss} displays the SST results for ID task performance (accuracy) \versus ER loss.
For a given ER criterion, each point in the corresponding scatter plot represents the checkpoint at some train epoch of the ER-trained model, evaluated on either the dev set or test set (yielding two point sets).
Fitting each point set with linear regression, we find that there is an inverse relationship between task performance and ER loss.
In other words, higher machine-human rationale alignment (\ie low ER loss) corresponds to higher task performance, which validates the usage of ER to improve generalization.
Table \ref{tab:exp:ext:loss} displays the slopes and $R^2$ scores of the lines in Fig. \ref{fig:exp:ext:loss}.
The slope indicates the strength of the relationship between machine-human rationale alignment and task performance (lower is better), while the $R^2$ score indicates how accurately each line fits its corresponding data points.
Among the five ER criteria, across dev and test, we find that MAE has the lowest slopes and highest $R^2$ scores overall, suggesting that using ER with MAE is most effective.
\paragraph{ER Opportunity Cost}
An ER-trained LM $\mathcal{F}_{\text{task, ER}}$ and a non-ER-trained LM $\mathcal{F}_{\text{task, No-ER}}$ are likely to yield different outputs given the same inputs.
Let $\mathcal{D}_{\text{ER}}^{+} \subseteq \mathcal{D}$ and $\mathcal{D}_{\text{No-ER}}^{+} \subseteq \mathcal{D}$ denote the sets of instances predicted correctly by $\mathcal{F}_{\text{task, ER}}$ and $\mathcal{F}_{\text{task, No-ER}}$, respectively.
Ideally, we would have $\mathcal{D}_{\text{No-ER}}^{+} \subset \mathcal{D}_{\text{ER}}^{+}$.
This means there is no \textit{opportunity cost} in using ER, as ER increases the number of correct instances without turning any previously-correct incorrect.
However, this may not necessarily be the case, so we measure ER's opportunity cost as follows.
Let $n_{\text{ER}}^{+} = | \mathcal{D}_{\text{ER}}^{+} \backslash (\mathcal{D}_{\text{ER}}^{+} \cap \mathcal{D}_{\text{No-ER}}^{+}) |$ be the number of instances predicted correctly by $\mathcal{F}_{\text{task, ER}}$, but not by $\mathcal{F}_{\text{task, No-ER}}$.
Let $n_{\text{No-ER}}^{+} = | \mathcal{D}_{\text{No-ER}}^{+} \backslash (\mathcal{D}_{\text{No-ER}}^{+} \cap \mathcal{D}_{\text{ER}}^{+}) |$ be the number of instances predicted correctly by $\mathcal{F}_{\text{task, No-ER}}$, but not by $\mathcal{F}_{\text{task, ER}}$.
Then, the opportunity cost of using ER is defined as:
\vspace{-0.1cm}
\begin{equation}
\label{eq:opp_cost}
\begin{split}
o_{\text{ER}} = \frac{n_{\text{No-ER}}^{+} - n_{\text{ER}}^{+}}{|\mathcal{D}|}
\end{split}
\end{equation}
In practice, instead of defining $o_{\text{ER}}$ for all of $\mathcal{D}$, we only consider test sets $\mathcal{D}_{\text{test}}$ and $\tilde{\mathcal{D}}_{\text{test}}$.
% \aaron{Check that this opportunity cost definition is correct.}
% \aaron{Do we plot for both ID and OOD?}

\begin{table*}[t!]
% \vspace{-0.2cm}
\centering
\scalebox{0.6}{
\begin{tabular}{ccccccc}
    \toprule
    \multirow{4}{*}{\textbf{ER criteria}} & \multicolumn{4}{c}{\textbf{Sentiment Analysis}} \\
    \cmidrule(lr){2-5}
    & In-Domain & \multicolumn{3}{c}{Out-of-Domain} \\
    \cmidrule(lr){2-2} \cmidrule(lr){3-5}
    & SST & Amazon & Yelp & Movies \\
    \midrule
    {None} & 0.00~($\pm$0.00) & 0.00~($\pm$0.00) & 0.00~($\pm$0.00) & 0.00~($\pm$0.00) \\
    \midrule
    {IxG+MSE} & 0.32~($\pm$1.05) & \textbf{-1.25~($\pm$1.20)} &\textbf{-2.33~($\pm$4.64)} & -6.50~($\pm$40.66) \\
    {IxG+MAE} & -0.09~($\pm$0.24) & -0.58~($\pm$3.45) & -0.94~($\pm$11.21) & \textbf{-7.00~($\pm$40.66)} \\
    {IxG+BCE} & \textbf{-0.16~($\pm$0.33)} & 0.46~($\pm$4.11) & 0.96~($\pm$26.99) & 0.16~($\pm$47.72) \\
    {IxG+Huber} & 0.12~($\pm$0.42) & 0.19~($\pm$2.25) & -1.05~($\pm$4.11) & -4.33~($\pm$37.72) \\
    {IxG+Order} & 1.90~($\pm$1.38) & 6.98~($\pm$3.87) & 19.86~($\pm$45.54) & 21.66~($\pm$35.72) \\
    
    \bottomrule 
\end{tabular}
}
% \vspace{0.3cm}
\caption{\small \textbf{ID/OOD Opportunity Cost.} Lower values are better.}
\label{tab:opp_cost}
% \vspace{-0.3cm}
\end{table*}

\begin{figure}[ht]
    \centering
    \includegraphics[width=0.9\linewidth]{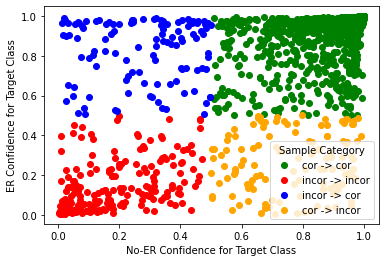}
    \vspace{-0.3cm}
    \caption{\small \textbf{Change in Target Class Confidence}} 
    \label{fig:exp:ext:conf}
\end{figure}
\begin{table}[]
\centering
\scalebox{0.5}{
\begin{tabular}{cccccccccc}
\toprule
\multicolumn{10}{c}{\textbf{Percentage of Dev Instances in $incor \hspace{-1mm} \rightarrow \hspace{-1mm} cor$ Group, Binned by} $\mathcal{F}_{\text{No-ER}}$ \textbf{Target Class Confidence}} \\
 \cmidrule(lr){1-10}
0.0-0.1 & 0.1-0.2 & 0.2-0.3 & 0.3-0.4 & 0.4-0.5 & 0.5-0.6 & 0.6-0.7 & 0.7-0.8 & 0.8-0.9 & 0.9-1.0 \\ 

\midrule

22.85 & 26.00 & 40.38 & 49.20 & 28.78 & 0.00 & 0.00 & 0.00 & 0.00 & 0.00 \\

\bottomrule

\end{tabular}}
\caption{\small \textbf{Change in Target Class Confidence.} For bins where $\mathcal{F}_{\text{No-ER}}$'s target class confidence is low, there is a higher percentage of instances that are predicted incorrectly/correctly without/with ER. This suggests that instances with low target class confidence are more likely to benefit from ER.}
\label{tab:exp:ext:conf}
\end{table}

\paragraph{Change in Target Class Confidence}
% Inspired by \citet{swayamdipta2020dataset}, for both $\mathcal{F}_{\text{ER}}$ and $\mathcal{F}_{\text{No-ER}}$, we plot ER loss $\mathcal{L_{\text{ER}}}$ as a function of the model's confidence in target class $\dot{y}_i$.
% Furthermore, each point in the plot is color-coded by target class and designated a marker w.r.t. whether ER changes the prediction from correct to incorrect, changes the prediction from incorrect to correct, keeps the prediction as correct, or keeps the prediction as incorrect.
% The purpose of this evaluation is to determine whether there is a predictive relationship between confidence and ER loss.
% If so, then we can use confidence as a feature for determining which instances are most/least likely to benefit from ER.
Let $\mathcal{F}_{\text{No-ER}}$ and $\mathcal{F}_{\text{ER}}$ denote non-ER-trained (vanilla) and ER-trained LMs, respectively.
For each test instance, we plot $\mathcal{F}_{\text{No-ER}}$'s predicted target class confidence probability \versus $\mathcal{F}_{\text{ER}}$'s.
Each point in the plot is color-coded by whether ER changes the prediction from correct to incorrect, changes the prediction from incorrect to correct, keeps the prediction as correct, or keeps the prediction as incorrect.
The purpose of this plot is to visualize how individual instances' predictions are affected by ER.
We conduct this for ID dev sets.\\

We consider ER with the MAE criterion, trained/evaluated on SST (via dev ID task performance). 
Fig. \ref{fig:exp:ext:conf} visualizes how ER changes each dev instance's target class confidence as a result of ER, color-coding each point with respect to how ER changes the model's predicted class for this point.
Among instances for which $\mathcal{F}_{\text{No-ER}}$'s target class confidence is low, there is a higher percentage of instances that are predicted incorrectly/correctly without/with ER (\ie $incor \hspace{-1mm} \rightarrow \hspace{-1mm} cor$). This suggests that, for $\mathcal{F}_{\text{No-ER}}$, instances with low target class confidence are more likely to benefit from ER (Table \ref{tab:exp:ext:conf}).
Also, based on the T-test, target class confidence scores are significantly higher ($p < 0.005$) with ER than without.

Table \ref{tab:opp_cost} displays the opportunity cost results for sentiment analysis.
Generally, the opportunity cost results mirror the task performance results in Table \ref{tab:exp:rq1:unseen}, such that the methods with highest task performance tend to have the lowest opportunity cost.
However, using opportunity cost, the variance is very high for OOD datasets, making it difficult to compare methods.
In future work, we plan to modify the opportunity cost metrics to better accommodate OOD settings.


% \aaron{Double check this.}


% \aaron{NLI/NER results go in appendix, if we have them.}


% \aaron{Update this.}
% \aaron{Make sure we have this result, since it's needed to motivate instance prioritization.}
% \aaron{Clarify which plot this is.}



% \aaron{For now, only doing SST+ID.}
% \aaron{Add NLI/NER results to appendix, if we have them.}



% \aaron{Add NER results.}

\subsubsection{Efficient hyperparameter tuning with \method}
% \label{sec:exp:use}
% To further show \method's utility, we conduct two pilot studies on low-resource learning: \textit{ER hyperparameter selection} (tuning budget) and \textit{ER instance prioritization} (rationale annotation budget).


% \subsubsection{ER Hyperparameter Selection}
\label{sec:app:use:hparam}

In intrinsic evaluation (\textsection \ref{sec:app:intrinsic_main}), we used ER loss curves as priors for selecting three key ER hyperparameters (\ie ER strength $\lambda_{\text{ER}}$, rationale scaling factor $\gamma_{\text{ER}}$, learning rate $\alpha$).
In \textsection \ref{sec:exp}, we assumed a tuning budget that allows only one value for each of $\lambda_{\text{ER}}$, $\gamma_{\text{ER}}$, and $\alpha$.
By not tuning these hyperparameters, we greatly reduced our hyperparameter search space.
Since ER has little effect on ID task performance, tuning based on ID task performance is unlikely to have helped anyway.
ER works better on OOD data, but it also does not make sense to tune based on OOD task performance (otherwise, it would not be OOD).
Though the ER hyperparameters chosen via intrinsic evaluation generally improved OOD task performance, we seek to verify their effectiveness compared to other possible hyperparameter values.

In Table \ref{tab:exp:use:hparam}, we report sentiment analysis OOD (Amazon, Yelp, Movies) task performance, while varying each of the three hyperparameters.
We include a Mean column, which averages the Amazon/Yelp/Movies columns.
Our hyperparameters chosen via ER loss curves are highlighted in \colorbox{lblue}{blue}.
For $\lambda_{\text{ER}}$, 1 (ours) and 100 yield very similar Mean results, while considerably beating the other three values.
For $\gamma_{\text{ER}}$, we see the same trend for 100 (ours) and 10.
For $\alpha$, $2\mathrm{e}{-5}$ (ours) vastly outperforms other values in all columns.
These results validate the utility of \method's intrinsic evaluation for low-resource ER hyperparameter tuning.
% In other words, how much better would the OOD task performance be if we had 
\subsection{RQ1}
\label{sec:app:rq1}
\begin{table}[ht]
\vspace{-0.2cm}
\hspace{-0.2cm}
\centering
\scalebox{0.75}{
\begin{tabular}{cccccccccc}
    \toprule
    Extractor & Criterion & SST & ESNLI\\
    \midrule
    \multirow{6}{*}{IxG} & {MSE} & 93.39~($\pm$0.93) & 78.66~($\pm$0.42) \\
    & {MAE} & 92.93~($\pm$0.24) & 78.46~($\pm$0.79)  \\
    & {BCE} & 93.35~($\pm$0.70) & 78.57~($\pm$0.81)\\
    & {Huber} & 92.89~($\pm$0.61) &  78.69~($\pm$0.29)  \\
    & {Order} & 90.83~($\pm$1.91) & 78.93~($\pm$0.74)  \\
    & {KlDiv} & 92.89~($\pm$0.30) & 73.41~($\pm$5.09)  \\
    \midrule
      \multirow{6}{*}{Attention} &  {MSE} & 93.27~($\pm$0.78) & 75.41~($\pm$0.42) \\
    & {MAE} & 93.65~($\pm$0.63) & 76.27~($\pm$0.92)  \\
    & {BCE} & 93.46~($\pm$0.90) & 75.55~($\pm$0.40)\\
    & {Huber} & 93.08~($\pm$0.07) &  75.98~($\pm$0.68)  \\
    & {Order} & 93.98~($\pm$0.08) & 75.99~($\pm$0.24)  \\
    & {KlDiv} & 93.50~($\pm$0.54) & 76.69~($\pm$0.49)  \\
    \midrule
    \multirow{6}{*}{UNIREX} & {MSE} & 92.43~($\pm$0.20) & 73.77~($\pm$1.81) \\
    & {MAE} & 93.31~($\pm$0.57) & 72.92~($\pm$1.45)  \\
    & {BCE} & 92.89~($\pm$0.11) & 68.81~($\pm$1.54)\\
    & {Huber} & 92.47~($\pm$0.76) &  73.33~($\pm$2.12)  \\
    & {Order} & 93.00~($\pm$0.23) & 72.26~($\pm$0.82)  \\
    & {KlDiv} & 92.43~($\pm$0.23) & 74.05~($\pm$1.20)  \\
    \bottomrule 
\end{tabular}
}
\caption{\small \textbf{RQ1 Performance on dev set} }
\label{tab:exp:ext:instance_prioritisation}
\vspace{-0.4cm}
\end{table}

\paragraph{NER Results}

We also have named entity recognition (NER) task, using CoNLL-2003 \cite{sang2003introduction, lin2020triggerner} as the ID dataset.
For the OOD dataset, we use OntoNotes v5.0 \cite{pradhan2013towards}.
CoNLL-2003 contains only Reuters news stories, while OntoNotes v5.0 contains text from newswires, magazines, telephone conversations, websites, and other sources.\\
In Table \ref{tab:app:task_perf_ner}, we display the ID and OOD results of NER. In ID, we see more variance in task performance among ER criteria, although the variance is still quite small among the best methods (MSE, MAE, Huber).
Here, MAE yields the highest task performance, while BCE yields the lowest by far. In OOD, MAE still performs best, while MSE and Huber are competitive.

\paragraph{Functional Tests} We provide details for different functional tests listen in \textsection \ref{sec:method:ood:functional}. We breakdown each subcategory of functional tests and show performances of different ER criteria on those individual tests. For functional tests on the sentiment analysis task, refer to Table \ref{tab:checklist:sst:ood}. NLI functional tests are listed in Table \ref{tab:checklist:nli:ood}. 
\begin{table*}[t!]
% \vspace{-0.2cm}
\centering
\scalebox{0.57}{
\begin{tabular}{cccccccc}
    \toprule
    \multirow{2}{*}{\textbf{Capability}} & \multirow{2}{*}{\textbf{Test Type}} & \multicolumn{6}{c}{\textbf{ER criteria}}\\
    \cmidrule(lr){3-8}
& & \textbf{None} & \textbf{IxG+MSE} & \textbf{IxG+MAE} & \textbf{IxG+BCE} & \textbf{IxG+Huber} & \textbf{IxG+Order} \\
\midrule
\multirow{6}{*}{\textbf{Vocabulary}} & Sentiment-laden words in context & 1.20~($\pm$0.74) & 0.60~($\pm$0.16) & 1.27~($\pm$0.84) & 1.00~($\pm$0.86) & 1.13~($\pm$0.50) & 0.80~($\pm$0.28) \\
& Change Neutral words with BERT & 5.59~($\pm$0.16) & 5.13~($\pm$0.90) & 5.40~($\pm$0.28) & 5.67~($\pm$0.68) &  5.67~($\pm$0.74) & 5.60~($\pm$1.63) \\
& Intensifiers & 2.13~($\pm$1.63) & 1.80~($\pm$0.16) & 1.40~($\pm$0.16) & 2.67~($\pm$0.77) & 2.67~($\pm$0.96) & 1.60~($\pm$0.65) \\
& Reducers & 23.85~($\pm$7.18) & 35.00~($\pm$46.01) & 27.38~($\pm$5.95) & 25.00~($\pm$25.00)  & 17.46~($\pm$13.65) & 0.77~($\pm$0.43) \\
& Add +ve phrases & 1.40~($\pm$0.28) & 2.33~($\pm$1.84) & 0.67~($\pm$0.50) & 1.27~($\pm$1.00) & 2.33~($\pm$1.76) & 2.07~($\pm$1.52)  \\
& Add -ve phrases & 22.86~($\pm$7.43) & 14.80~($\pm$1.40) & 20.67~($\pm$4.07) & 17.40~($\pm$3.64) &20.67~($\pm$3.35) & 16.93~($\pm$1.91) \\
\midrule
\multirow{5}{*}{\textbf{Robustness}} & Adding Random URLs and Handles & 9.80~($\pm$0.48) & 7.27~($\pm$2.23) & 9.07~($\pm$1.80) & 7.87~($\pm$2.76) & 10.27~($\pm$0.9) & 9.6~($\pm$2.47) \\
& Punctuations & 3.93~($\pm$0.89) & 1.93~($\pm$0.41) & 3.00~($\pm$1.02) & 2.87~($\pm$0.19) & 3.80~($\pm$0.28) & 2.67~($\pm$0.34) \\
& Typos & 2.60~($\pm$0.90) & 2.53~($\pm$0.82) & 2.60~($\pm$0.57) & 3.13~($\pm$0.90) & 2.60~($\pm$0.75) & 2.00~($\pm$0.86) \\
&2 Typos & 3.93~($\pm$0.65) & 3.87~($\pm$1.24) & 4.27~($\pm$0.5) & 4.13~($\pm$1.2) & 4.6~($\pm$0.43) & 3.33~($\pm$0.25) \\
& Contractions & 1.00~($\pm$0.00) & 0.80~($\pm$0.33) & 0.87~($\pm$0.25) & 0.80~($\pm$0.43) & 0.47~($\pm$0.09) & 0.53~($\pm$0.50) \\
\midrule
\multirow{3}{*}{\textbf{Logic}} & Negatives & 5.20~($\pm$2.75)  & 4.27~($\pm$1.65)  & 4.47~($\pm$3.07)  & 4.47~($\pm$1.75) & 3.93~($\pm$1.57) & 5.67~($\pm$1.68)\\
& Non-negatives & 59.73~($\pm$9.48) & 59.00~($\pm$15.81)  & 37.47~($\pm$10.41)  & 63.27~($\pm$17.61) & 59.07~($\pm$14.97) & 45.87~($\pm$24.13) \\
& Negation of positive with neutral stuff in the middle & 32.2~($\pm$14.65)  & 35.13~($\pm$1.91) & 35.00~($\pm$16.52)& 19.00~($\pm$8.66)  & 40.93~($\pm$4.31) & 29.13~($\pm$10.60)  \\
\midrule
\multirow{3}{*}{\textbf{Entity}} & Change Names &  0.70~($\pm$0.14 & 1.91~($\pm$0.71) & 1.11~($\pm$0.51) &  0.81~($\pm$0.14) & 1.61~($\pm$0.62) & 1.91~($\pm$1.51)  \\
& Change Locations & 3.33~($\pm$0.74) & 2.73~($\pm$1.15) & 3.40~($\pm$0.86) & 3.07~($\pm$1.79) & 3.00~($\pm$0.33) & 3.20~($\pm$1.57) \\
& Change Numbers & 0.80~($\pm$0.00) & 0.53~($\pm$0.34) &  0.47~($\pm$0.41) & 0.60~($\pm$0.33) & 0.60~($\pm$0.43) &  0.67~($\pm$0.81)\\
\bottomrule 
\end{tabular}
}
% \vspace{0.3cm}
\caption{\small \textbf{RQ1 - Functional Tests:} Sentiment Analysis}
\label{tab:checklist:sst:ood}
% \vspace{-0.3cm}
\end{table*}


% \begin{table}[t]
%     \centering
%     \scalebox{0.65}{
%     \begin{tabular}{cccccccccc}
%     \toprule
%     \multirow{4}{*}{\textbf{Method}}& \multirow{4}{*}{\textbf{ER Criteria}} & \multicolumn{4}{c}{\textbf{Sentiment Analysis}}  \\
%     \cmidrule(lr){3-5} 
%     & &{Original} & {Contrast} & {Delta} \\
%     \cmidrule(lr){3-3} \cmidrule(lr){4-4} \cmidrule(lr){5-5} 
  
%     \multirow{2}{*}{Lexicon} & {IxG+MAE} & 91.46~($\pm$0.72) & 89.82~($\pm$2.46) & -1.64 \\
%     & {IxG+Huber} & 90.64~($\pm$1.25) & 88.52 ~($\pm$2.25) & -2.12 & \\
%     \multirow{2}{*}{Instance} & {IxG+MAE} & 91.12~($\pm$0.59) & 89.82~($\pm$1.20) & -1.3 \\
%     & {IxG+Huber} & 89.20~($\pm$1.67) & 86.13 ~($\pm$1.74) & -3.15 & \\
   
%     \bottomrule 
%     \end{tabular}
%     }
   
%     \caption{\textbf{Contrast Set Tests:} Lexicon-based VS Instance-based. We use }
%     \label{tab:lexicon_contrast}
% \end{table}

% \begin{table}[t]
% \centering
% \scalebox{0.70}{
% \begin{tabular}{ccccccccc}
% \toprule
% \textbf{Capability}&Vocabulary&Robustness&Logic&Entity&Overall\\
% \midrule
% \textbf{Lexicon}&10.11&4.21&32.27&2.28&12.22\\
% \textbf{Instance}&11.90&3.574&30.2&1.86&11.89\\
% \bottomrule
% \end{tabular}

% }
% \caption{\textbf{Functional Tests:} Lexicon-based VS Instance-based. Here we use MAE criterion and  IxG as rationale extractor.}
% \label{tab:lexicon_functional}
% \end{table}

\begin{table*}[t!]
% \vspace{-0.2cm}
\centering
\scalebox{0.6}{
\begin{tabular}{cccccccc}
    \toprule
    \multirow{2}{*}{\textbf{Capability}} & \multirow{2}{*}{\textbf{Test Type}} & \multicolumn{6}{c}{\textbf{ER criteria}}\\
    \cmidrule(lr){3-8}
& & \textbf{None} & \textbf{IxG+MSE} & \textbf{IxG+MAE} & \textbf{IxG+BCE} & \textbf{IxG+Huber} & \textbf{IxG+Order} \\
\midrule
\multirow{3}{*}{\textbf{Vocabulary}} & Antonym in Hypothesis & 71.66~($\pm$20.98) & 64.77~($\pm$21.97) & 84.55~($\pm$11.53) & 65.88~($\pm$21.40) & 74.77~($\pm$20.41) & 62.55~($\pm$13.16) \\
& Synonym in Hypothesis & 32.61~($\pm$7.41) & 24.11~($\pm$7.62) & 30.11~($\pm$6.42) & 25.88~($\pm$6.86) & 30.77~($\pm$7.07) & 29.27~($\pm$6.95) \\
& Supertype in Hypothesis & 24.44~($\pm$15.95) & 11.00~($\pm$3.62) & 13.77~($\pm$6.71) & 9.31~($\pm$5.90) & 8.77~($\pm$8.06) & 13.55~($\pm$7.10) \\
\midrule
\multirow{4}{*}{\textbf{Robustness}} & Punctuation & 14.55~($\pm$4.13) & 9.44~($\pm$2.79) & 11.33~($\pm$1.63) & 8.11~($\pm$1.19) & 10.00~($\pm$2.58) & 9.88~($\pm$2.51) \\
& Typo & 15.88~($\pm$3.44) & 10.22~($\pm$3.04) & 12.33~($\pm$1.63) & 9.66~($\pm$2.10) & 10.88~($\pm$2.68) & 10.77~($\pm$2.52) \\
& 2 Typos & 15.33~($\pm$3.68) & 9.77~($\pm$1.81) & 12.00~($\pm$1.76) & 9.44~($\pm$2.31) & 11.11~($\pm$2.99) & 10.00~($\pm$2.66) \\
& Contractions & 24.69~($\pm$6.98) & 24.69~($\pm$8.72) & 25.92~($\pm$9.07) & 22.22~($\pm$9.07) & 25.92~($\pm$7.40) & 14.81~($\pm$5.23) \\
\midrule
\multirow{3}{*}{\textbf{Logic}} &Negation in the Hypothesis & 50.88~($\pm$32.25) & 27.77~($\pm$37.24) & 9.77~($\pm$15.66) & 41.33~($\pm$41.54) & 15.22~($\pm$28.77) & 18.44~($\pm$23.21) \\
& Induce Contradiction & 99.88~($\pm$0.31) & 98.54~($\pm$3.78) & 91.69~($\pm$20.37) & 98.65~($\pm$2.56) & 98.42~($\pm$4.44) & 99.88~($\pm$0.31) \\
& Same Premise and Hypothesis & 14.22~($\pm$8.63) & 14.33~($\pm$10.14) & 19.44~($\pm$12.12) & 18.16~($\pm$12.69) & 14.38~($\pm$9.23) & 17.38~($\pm$10.16) \\
\midrule
\multirow{1}{*}{\textbf{Entity}} & Switch one Entity in the Hypothesis & 77.21~($\pm$39.57) & 88.88~($\pm$24.11) & 79.91~($\pm$22.20) & 85.18~($\pm$30.04) & 83.83~($\pm$24.25) & 96.40~($\pm$4.85) \\
\bottomrule 
\end{tabular}
}
% \vspace{0.3cm}
\caption{\small \textbf{RQ1 - Functional Tests:} NLI}
\label{tab:checklist:nli:ood}
% \vspace{-0.3cm}
\end{table*}

\begin{figure*}[t!]
\vspace{-0.2cm}
\centering
\includegraphics[width=\linewidth]{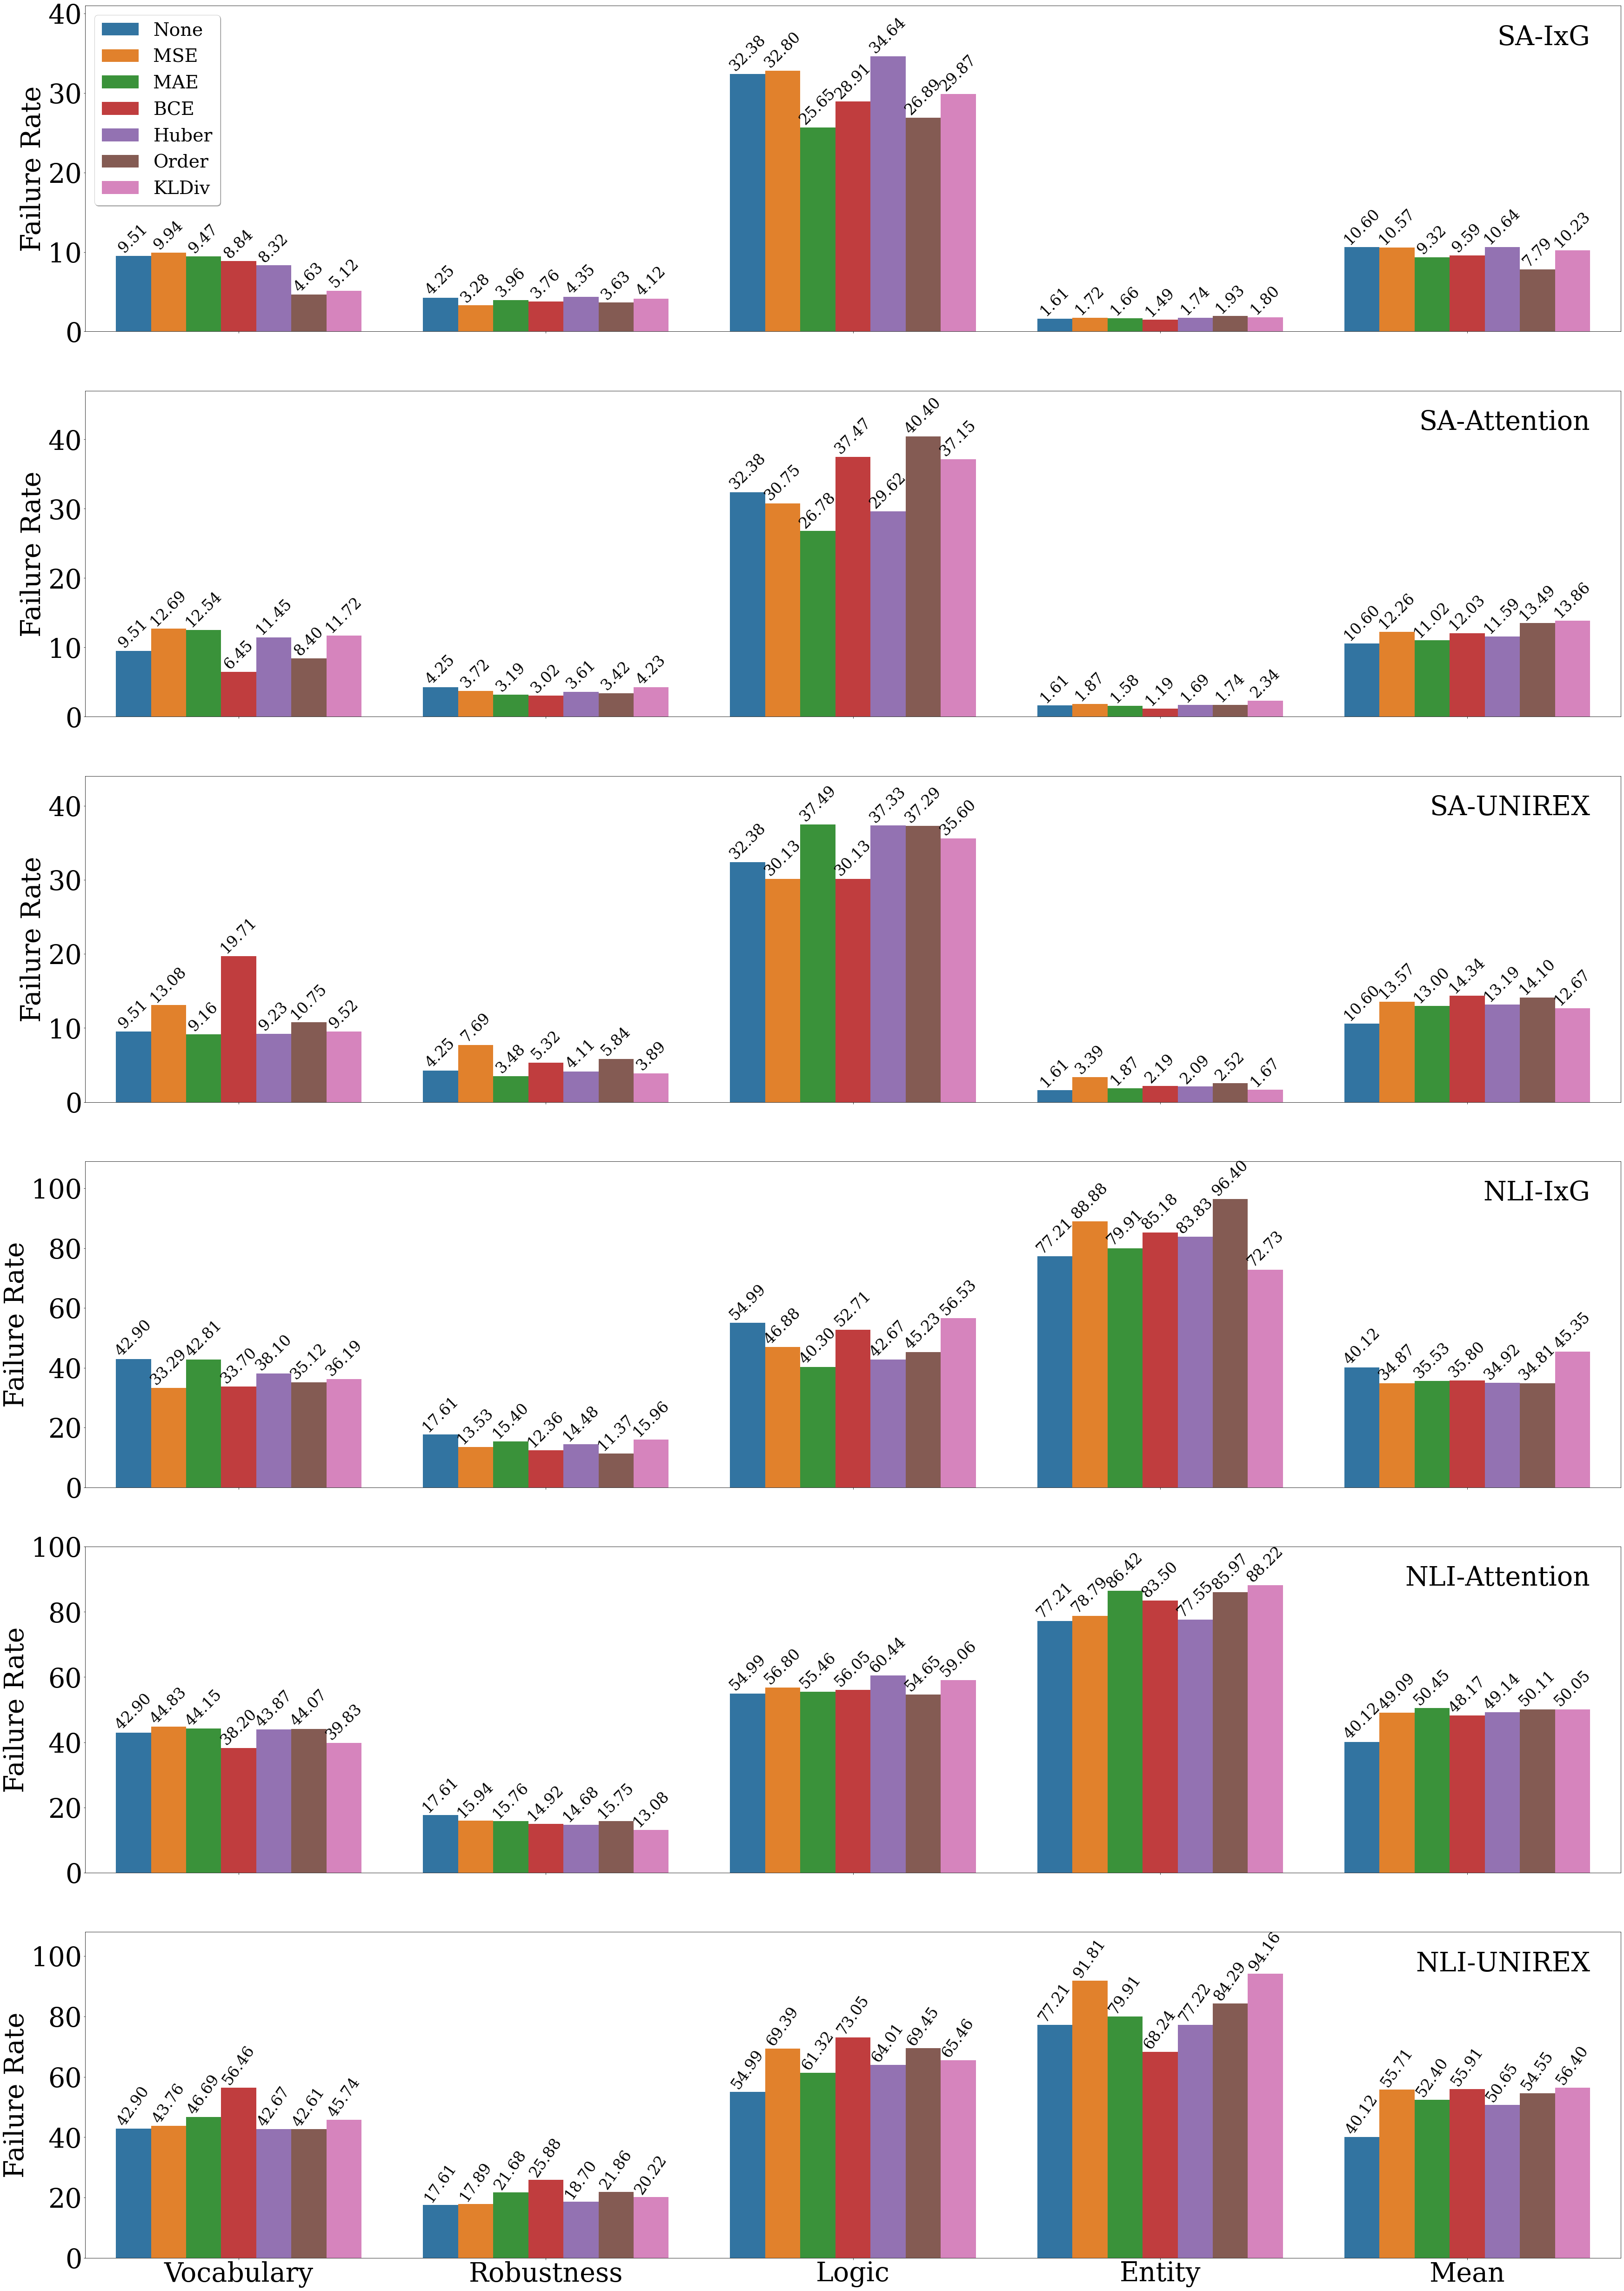}
\vspace{-0.3cm}
\caption{\small \textbf{RQ1 - Functional Tests' Failure Rates (lower the better):} We plot the failure rates of the four functional tests (vocab., robust., logic, entity) as described in \textsection \ref{sec:method:ood:functional}, as well as the overall failure rate on all of the tests combined (mean). Each of the values are out of 100, but plotted accordingly for visible comparison. Here we use IxG as rationale extractor.
}
\label{fig:exp:rq1:functional_apx}
\end{figure*}

\begin{table}[t]
% \vspace{-0.2cm}
\centering
\scalebox{0.60}{
\begin{tabular}{ccccccccc}
    \toprule
    \multirow{4}{*}{\textbf{Methods}} & \multicolumn{2}{c}{\textbf{NER}} \\
   \cmidrule(lr){2-3}
  & In-Distribution & \multicolumn{1}{c}{Out-of-Distribution} \\
 \cmidrule(lr){2-2} \cmidrule(lr){3-3} &
    CoNLL-2003 & OntoNotes v5.0\\
    \midrule
    {None} & 77.24~($\pm$0.20) & 20.78~($\pm$0.41)\\
    \midrule
    {IxG+MSE}  & 78.02~($\pm$0.69) & 21.60~($\pm$0.46)\\
    {IxG+MAE}  & \textbf{78.34~($\pm$0.81)} & \textbf{21.73~($\pm$0.31)}\\
    {IxG+BCE} & 64.53~($\pm$13.22) & 17.32~($\pm$3.59)\\
    {IxG+Huber} & 77.83~($\pm$1.09) & 21.38~($\pm$0.16)\\
    {IxG+Order} & 72.62~($\pm$5.01) & 19.14~($\pm$1.75)\\ 
    
    
    \bottomrule 
\end{tabular}
}
% \vspace{0.3cm}
\caption{\small \textbf{RQ1 - Unseen Dataset Tests on NER (Instance-Based Human Rationales).}
}
\label{tab:app:task_perf_ner}
% \vspace{-0.3cm}
\end{table}


\subsection{RQ2}

\subsubsection{Lexicon-matching}
\label{sec:app:lexicon_matching}
\begin{table}[ht]
\vspace{-0.2cm}
\centering
\scalebox{0.75}{
\begin{tabular}{cccccccccc}
    \toprule
    Extractor & Criterion & Accuracy \\
    \midrule
    \multirow{2}{*}{IxG} & {MAE} &  93.46~($\pm$0.11)  \\
    & {Huber} &  93.27~($\pm$0.48) \\
   \multirow{2}{*}{Attention} & {MAE} &  94.31~($\pm$0.71)  \\
    & {Huber} &  93.98~($\pm$0.33) \\
    \multirow{2}{*}{UNIREX} & {MAE} &  92.34~($\pm$1.11)  \\
    & {Huber} &  93.45~($\pm$0.86) \\
 
    \bottomrule 
\end{tabular}
}
\caption{\small \textbf{RQ2 Lexicon-based Performance on dev set} }

\label{tab:exp:ext:lexicon_based_dev_performance}
\vspace{-0.4cm}
\end{table}
% \begin{table}[ht]
% \vspace{-0.2cm}
% \centering
% \scalebox{0.60}{
% \begin{tabular}{cccccccccc}
%     \toprule
%     Extractor & Criterion & Original & Contrast & $\Delta$ & consistency\\
%     \midrule
%     \multirow{2}{*}{IxG} & {MAE} &  91.46~($\pm$0.72) &89.82~($\pm$2.46) & 1.64 &\cellcolor{lblue}83.47~($\pm$0.47) \\
%     & {Huber} &  90.64~($\pm$1.25) &89.82~($\pm$2.46) & 0.84 &\cellcolor{lblue}79.58~($\pm$1.72) \\
%    \multirow{2}{*}{Attention} & {MAE} &  91.19~($\pm$0.20) & 91.94~($\pm$0.43) & 0.75&\cellcolor{lblue}83.47~($\pm$0.47)\\
%     & {Huber} &  91.12~($\pm$0.12) & 91.94~($\pm$0.43) &0.82& \cellcolor{lblue}79.58~($\pm$2.07)\\
%     \multirow{2}{*}{UNIREX} & {MAE} &  84.77~($\pm$9.03)&  77.94~($\pm$13.45) & 6.83 & 62.98 ~($\pm$22.43)\\
%     & {Huber} &  89.89~($\pm$0.52) & 84.02~($\pm$1.55) & 5.87 &74.25~($\pm$2.17) \\
 
%     \bottomrule 
% \end{tabular}
% }
% \caption{\small \textbf{RQ2 Lexicon-based contrast set results} }
% \label{tab:exp:ext:lexicon_based_contrast}
% \vspace{-0.4cm}
% \end{table}
Let $\mathcal{L}_{\mathcal{D}}$ be a list of lexicons curated by human annotators, specific to a given dataset $\mathcal{D}$. 
Let $l(\cdot)$ be an indicator function that searches for a given lexicon list in all the tokens of an instance, and returns a binary representation of the same size as the instance with $1$s in places with lexicon matches ($0$ otherwise). 
Therefore, we can obtain distantly-supervised human rationales $\mathbf{\dot{r}}_{i} = l(\mathcal{L}_{\mathcal{D}}, x_{i})$ and apply rationale alignment criteria as described in \textsection \ref{sec:eval:er_criteria}.

Each lexicon is matched to n-grams(uni-/bi-/tri-grams), which leads to 93\% of the train set instances to be matched. Additionally, since we combined two lexicons as resources, there are words appeared as important and unimportant. We maintain lexicon overlapping with different sentiment polarities when matching with tokens.
For equal comparison, we use instance-based rationales on the same train subset.
% We also run contrast set tests and functional tests on both lexicon-based and instance-based methods. The results are shown in Table \ref{tab:exp:ext:lexicon_based_contrast} and Table \ref{tab:lexicon_functional}.

\subsubsection{Hate Speech Detection Tests}
\label{sec:app:hate_speech}

\paragraph{Task-Level Rationales}

For example, \citet{kennedy2020contextualizing} used a ``blacklist'' lexicon to distantly supervise human rationales for the hate speech detection task.
In the past, hate speech detection models were largely oversensitive to certain group identifier words (\eg ``black'', ``Muslim'', ``gay''), almost always predicting hate speech for text containing these words.
To address this, they first manually annotated a lexicon of group identifiers that should be ignored for hate speech detection.
Then, for all training instances, they automatically marked only tokens belonging to the lexicon as unimportant (and the rest as important).
By using these human rationales for ER, they trained the LM to be less biased with respect to these group identifiers. 
For the purpose of our study, we use the lexicons as used by \cite{jin-etal-2021-transferability} to generate distantly-supervised rationales for the Stormfromt (Stf) dataset \cite{de-gibert-etal-2018-hate}. Each instance in the Stf dataset is matched to one or more lexicons by simple character-level matching, and the rationales are generated as described above. We train $\mathcal{F}$ with the Stf dataset. We report all accuracies in Table \ref{tab:exp:ext:hate_results}. As it was observed in \textsection \ref{sec:exp:rq1}, ER does not lead to a significant improvement in performance for the Stf test set. However, it is important to note that ``blacklisting'' group identifier lexicons does not lead to a drop in ID performance either. Benefits of ``blacklisting'' are then observed in OOD generalization. We evaluate ER methods on OOD hate speech detection datasets like HatEval \cite{barbieri-etal-2020-tweeteval} and Gab Hate Corpus (GHC) \cite{kennedyghc}. All of the datasets contain binary labels for hateful and non-hateful content. The Stf dataset is collected from a white-supremacist forum, whereas HatEval instances are tweets and GHC instances are taken from the Gab forum. Table \ref{tab:exp:ext:hate_results} shows that while the improvements in HatEval are not significant, there are significant accuracy improvements for the GHC test set, which are due to the Order ER criterion. \\

\paragraph{Fairness Tests} In addition to generic performance metrics like accuracy, we also measure group identifier bias (against the groups detailed by group identifier lexicons) by evaluating the False Positive Rate Difference (FPRD) as shown by \cite{jin-etal-2021-transferability}. FPRD is computed as $\sum_{z} |\text{FPR}_{z} - \text{FPR}_{\text{overall}}|$, where $\text{FPR}_{z}$ is the false positive rate of all of the test instances mentioning group identifier $z$, and $\text{FPR}_{\text{overall}}$ is the false positive rate of all the test instance. Essentially, FPRD evaluates if $\mathcal{F}$ is more biased against a given group identifier $z$, than all of the groups. A lower FPRD value indicates less biased against the listed group identifiers by $\mathcal{F}$. 

Table \ref{tab:exp:ext:hate_results} lists the FPRD values of all the ER criteria in ID and OOD datasets. While all other criteria suffer with higher bias than None, we observe that Order criterion consistently leads to the least bias, both in-distribution and out-of-distribution. Furthermore, the reduction in bias is significant when compared to None. Interestingly, Order ER criterion was initially conceived for distantly-supervised rationales \cite{huang2021exploring}, and the authors of the original paper also demonstrated experiments with rationales generated from lexicons where Order criterion leads to improvements. Our observations are in-line with theirs, and we also show its benefit in reducing bias in $\mathcal{F}$.
\begin{table}[t]
% \vspace{-0.2cm}
\centering
\scalebox{0.45}{
\begin{tabular}{ccccccc}
    \toprule
    \multirow{5}{*}{\textbf{ER Criteria}} & \multicolumn{6}{c}{\textbf{Hate Speech Detection}} \\
    \cmidrule(lr){2-7}
    & \multicolumn{2}{c}{\textbf{In-Distribution}} & \multicolumn{4}{c}{\textbf{Out-of-Distribution}}\\
    \cmidrule(lr){2-3} \cmidrule(lr){4-7}
    &\multicolumn{2}{c}{Stf} & \multicolumn{2}{c}{HatEval} & \multicolumn{2}{c}{GHC} \\
    \cmidrule(lr){2-3} \cmidrule(lr){4-5} \cmidrule(lr){6-7}
    & Accuracy~$\uparrow$ & FPRD~$\downarrow$ & Accuracy~$\uparrow$ & FPRD~$\downarrow$ & Accuracy~$\uparrow$ & FPRD~$\downarrow$ \\
    \midrule
    {None} & 89.50~($\pm$0.20) & 1.11~($\pm$0.58) & 63.68~($\pm$0.78) & 1.64~($\pm$0.66) & 89.43~($\pm$0.98) & 1.09~($\pm$0.12)\\
    \midrule
    {IxG+MSE}  & 89.46~($\pm$0.21) & 2.18~($\pm$0.47) & 64.30~($\pm$1.52) & 1.99~($\pm$0.26) & 88.19~($\pm$0.62) & 1.50~($\pm$0.10)\\
    {IxG+MAE}  & \textbf{89.59~($\pm$0.06)} & 1.39~($\pm$0.62) & 63.30~($\pm$0.49) & 1.80~($\pm$0.59) & 88.07~($\pm$1.66) & 1.43~($\pm$0.24)\\
    {IxG+BCE} & 89.42~($\pm$0.71) & 1.87~($\pm$0.45) & 63.54~($\pm$0.57) & 1.87~($\pm$0.45) & 88.99~($\pm$0.83) & 1.36~($\pm$0.58)\\
    {IxG+Huber} & 89.50~($\pm$0.51) & 1.90~($\pm$0.35) & \textbf{64.85~($\pm$1.50)} & 2.11~($\pm$0.27) & 87.77~($\pm$1.21) & 1.84~($\pm$0.34)\\
    {IxG+Order} & 89.21~($\pm$1.18) & \textbf{0.56~($\pm$0.09)} & 64.46($\pm$1.18) & \textbf{0.92~($\pm$0.92)} & \textbf{92.84~($\pm$0.46)} & \textbf{0.59~($\pm$0.25)}\\
    
    \bottomrule 
\end{tabular}
}
% \vspace{0.3cm}
\caption{\small \textbf{RQ2 - Unseen Dataset Tests (Distantly-supervised Human Rationales)}: Higher values for accuracy and lower values for FPRD are considered better. All models displayed are trained on the ID dataset (Stf) with distantly supervised rationales (for ER criteria) and no rationales (for None) and evaluated on ID and OOD test splits.}
\label{tab:exp:ext:hate_results}
% \vspace{-0.3cm}
\end{table}
\subsection{RQ3}
\subsubsection{Details for Instance Prioritisation Experiments}
\label{sec:app:instance_prior}
In this section, we provide further implementation details for confidence-based instance prioritisation experiments as described in \textsection \ref{sec:eval:inst_select}. 
\begin{table}[ht]
\vspace{-0.2cm}
\hspace{-0.2cm}
\centering
\scalebox{0.75}{
\begin{tabular}{cccccccccc}
    \toprule
    k\% & Method & SST \\
    \midrule
    \multirow{5}{*}{5} & {Random} & 93.58~($\pm$0.23)  \\
    & {LC} & 92.55~($\pm$0.72)   \\
    & {HC} & 93.08~($\pm$0.35) \\
    & {LIS} & 92.62~($\pm$0.40) \\
    & {HIS} & 92.97~($\pm$0.52)  \\
    \midrule
      \multirow{5}{*}{15} 
      &  {Random} & 93.08~($\pm$0.28)  \\
    & {LC} & 92.24~($\pm$0.78)   \\
    & {HC} & 92.58~($\pm$0.46) \\
    & {LIS} & 93.08~($\pm$0.66) \\
    & {HIS} & 93.31~($\pm$0.18)  \\
    \midrule
    \multirow{5}{*}{50} 
      &  {Random} & 92.29~($\pm$0.06)  \\
    & {LC} & 87.58~($\pm$5.11)   \\
    & {HC} & 92.62~($\pm$0.81) \\
    & {LIS} & 92.24~($\pm$0.54) \\
    & {HIS} & 92.51~($\pm$0.37)  \\
    \bottomrule 
\end{tabular}
}
\caption{\small \textbf{RQ3 Performance on dev set}: we only consider the best instance priortization setting (LIS + 5\%) }
\label{tab:exp:ext:instance_prioritisation_dev_performace}
\vspace{0.4cm}
\end{table}


Given that we have $3$-seed runs for the None model in Table \ref{tab:exp:rq1:unseen}, we extract the confidence scores based on the given metric (LC/HC/LIS/HIS), and then average these confidence/importance scores across the $3$ seed runs to obtain a single score for every instance. This process is done for training set instances only. This is followed by ranking each instance by the aggregated confidence metric and selecting the top $k\%$ of samples from this ranking. For experiments with random sampling based prioritisation, we generate $3$ random subsets selected in a uniform manner. 

While training in this setting, we ensure that within each batch, certain (one third to be specific) set of instances have available rationales. For these instances, we calculate the ER loss $\mathcal{L}_{\text{ER}}$, whereas, for the rest of the instances in the batch, we compute the task loss $\mathcal{L}_{task}$. All prioritisation settings are trained with $3$ different model seeds and the aggregated results for ID and OOD datasets are shown in Table \ref{tab:exp:ext:instance_prioritisation}.




\subsection{RQ4}
\label{sec:app:time_budget}
\subsubsection{MTurk Annotation}
In this section, we demonstrate the MTurk experiment setup. 
Each MTurk annotator is paid minimum wage. Figures \ref{fig:app:rq4:task1}, \ref{fig:app:rq4:task2} and \ref{fig:app:rq4:task3} demonstrate UIs used by MTurk annotators for time-budget experiments.



\vspace{-0.4cm}
\begin{table}[ht]
% \vspace{-0.2cm}

\centering
\scalebox{0.75}{
\begin{tabular}{cccccccccc}
    \toprule
    Task & Time Budget & SST \\
    \midrule
    No Annotation&None&91.00~($\pm$0.18)\\
    \midrule
    \multirow{7}{*}{Label+Expl} & {10 min} &  90.66~($\pm$0.27)  \\
    & {30 min} &  91.08~($\pm$0.18) \\
    & {1 hr} & 91.46~($\pm$0.51) \\
    & {5 hr} & 91.30~($\pm$0.70) \\
    & {12 hr} & 92.16~($\pm$0.31)  \\
     & {24 hr} & 91.97~($\pm$0.53)  \\
      & {48 hr} & 92.37~($\pm$0.53)  \\
    \midrule
      \multirow{7}{*}{Only Expl} &
      {10 min} &  91.50~($\pm$0.31)  \\
    & {30 min} &  91.23~($\pm$0.21) \\
    & {1 hr} & 91.14~($\pm$0.23) \\
    & {5 hr} & 90.86~($\pm$0.77) \\
    & {12 hr} & 91.24~($\pm$0.06)  \\
     & {24 hr} & 91.24~($\pm$0.06)  \\
      & {48 hr} & 91.24~($\pm$0.06)  \\
    \midrule
    \multirow{7}{*}{Only Label} 
     &
      {10 min} &  91.09~($\pm$0.18)  \\
    & {30 min} &  90.88~($\pm$0.66) \\
    & {1 hr} & 91.04~($\pm$0.06) \\
    & {5 hr} & 91.62~($\pm$0.32) \\
    & {12 hr} & 91.42~($\pm$0.34)  \\
     & {24 hr} & 92.42~($\pm$0.67)  \\
      & {48 hr} & 92.70~($\pm$0.47)  \\
    \bottomrule 
\end{tabular}
}
\caption{\small \textbf{RQ4 Performance on dev set} }
\label{tab:exp:ext:time_budget_dev_performance}
\vspace{-0.4cm}
\end{table}

\begin{figure*}[ht]
    \centering
    \includegraphics[width=0.95\linewidth]{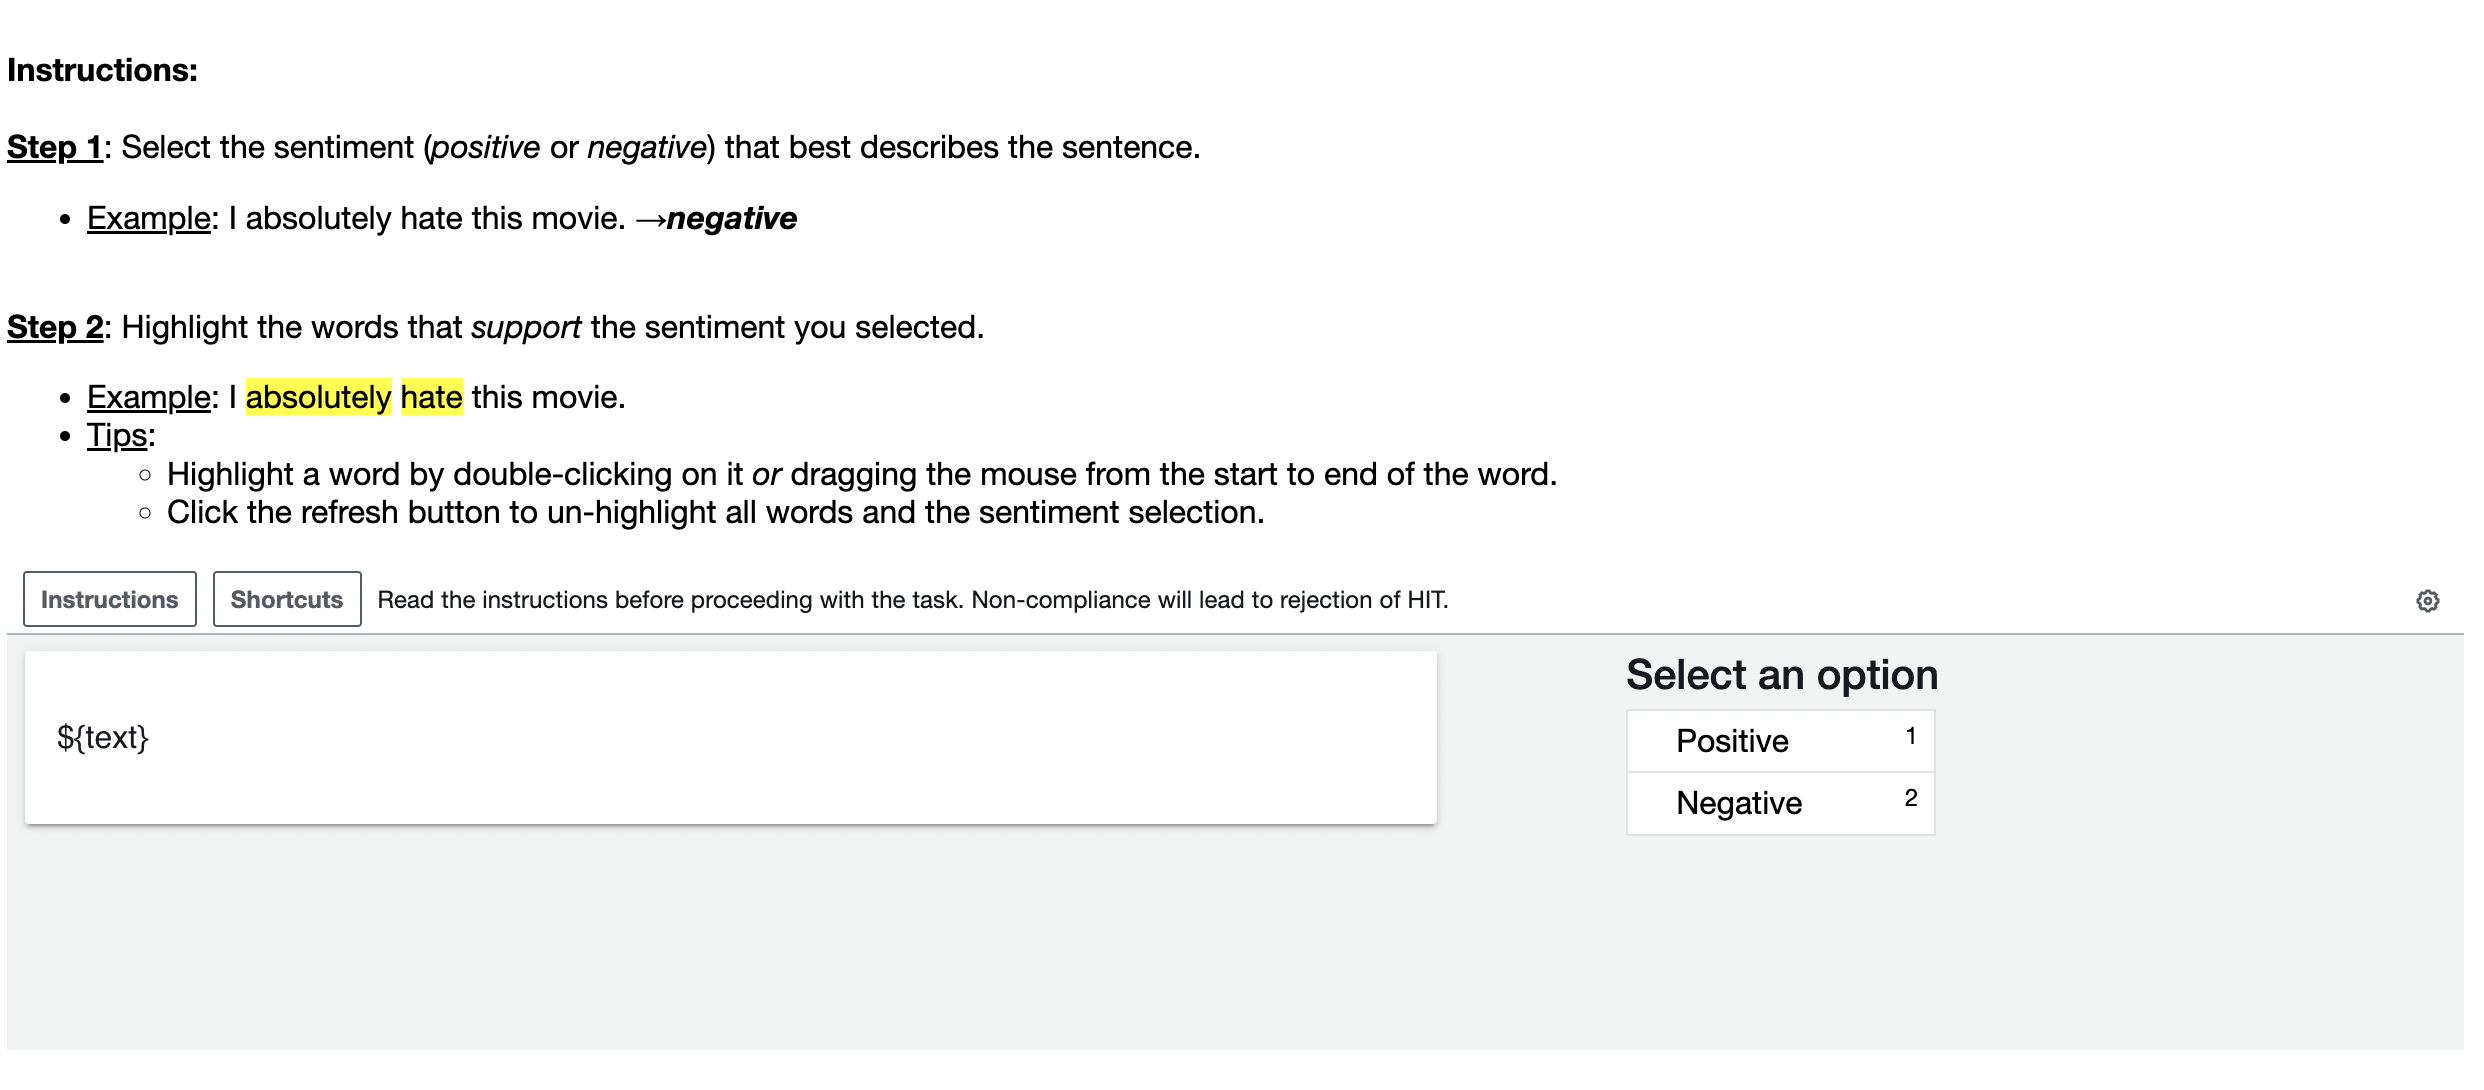}
    \caption{\textbf{Label + Expl:} Instructions and setup for Label + Expl annotation}
    \label{fig:app:rq4:task1}
\end{figure*}

\begin{figure*}[ht]
    \centering
    \includegraphics[width=0.95\linewidth]{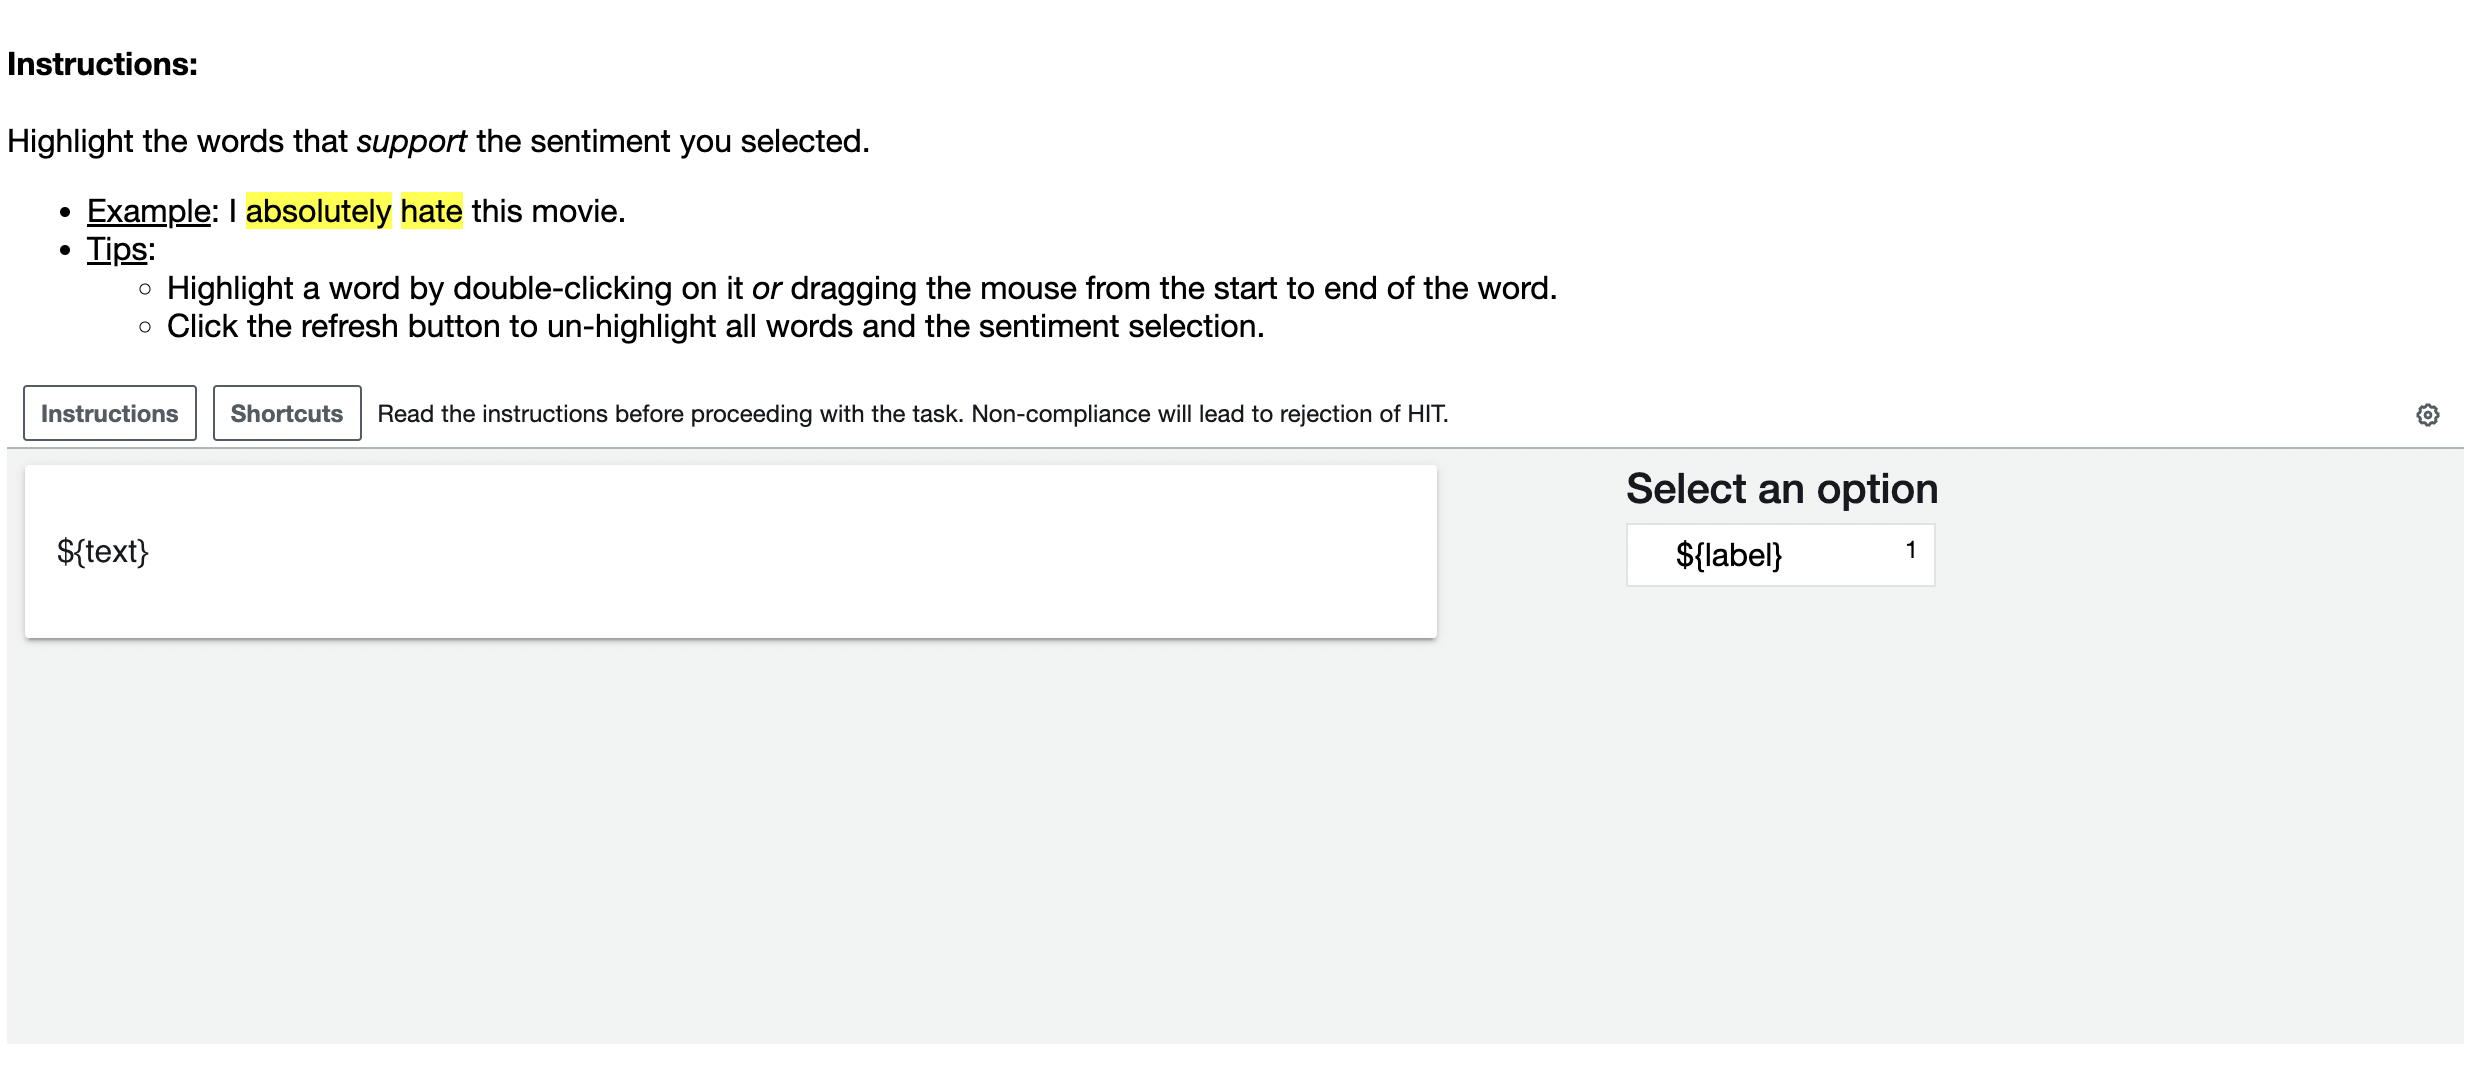}
    \caption{\textbf{Only Expl:} Instructions and setup for Only Expl annotation}
    \label{fig:app:rq4:task2}
\end{figure*}


\begin{figure*}[ht]
    \centering
    \includegraphics[width=0.95\linewidth]{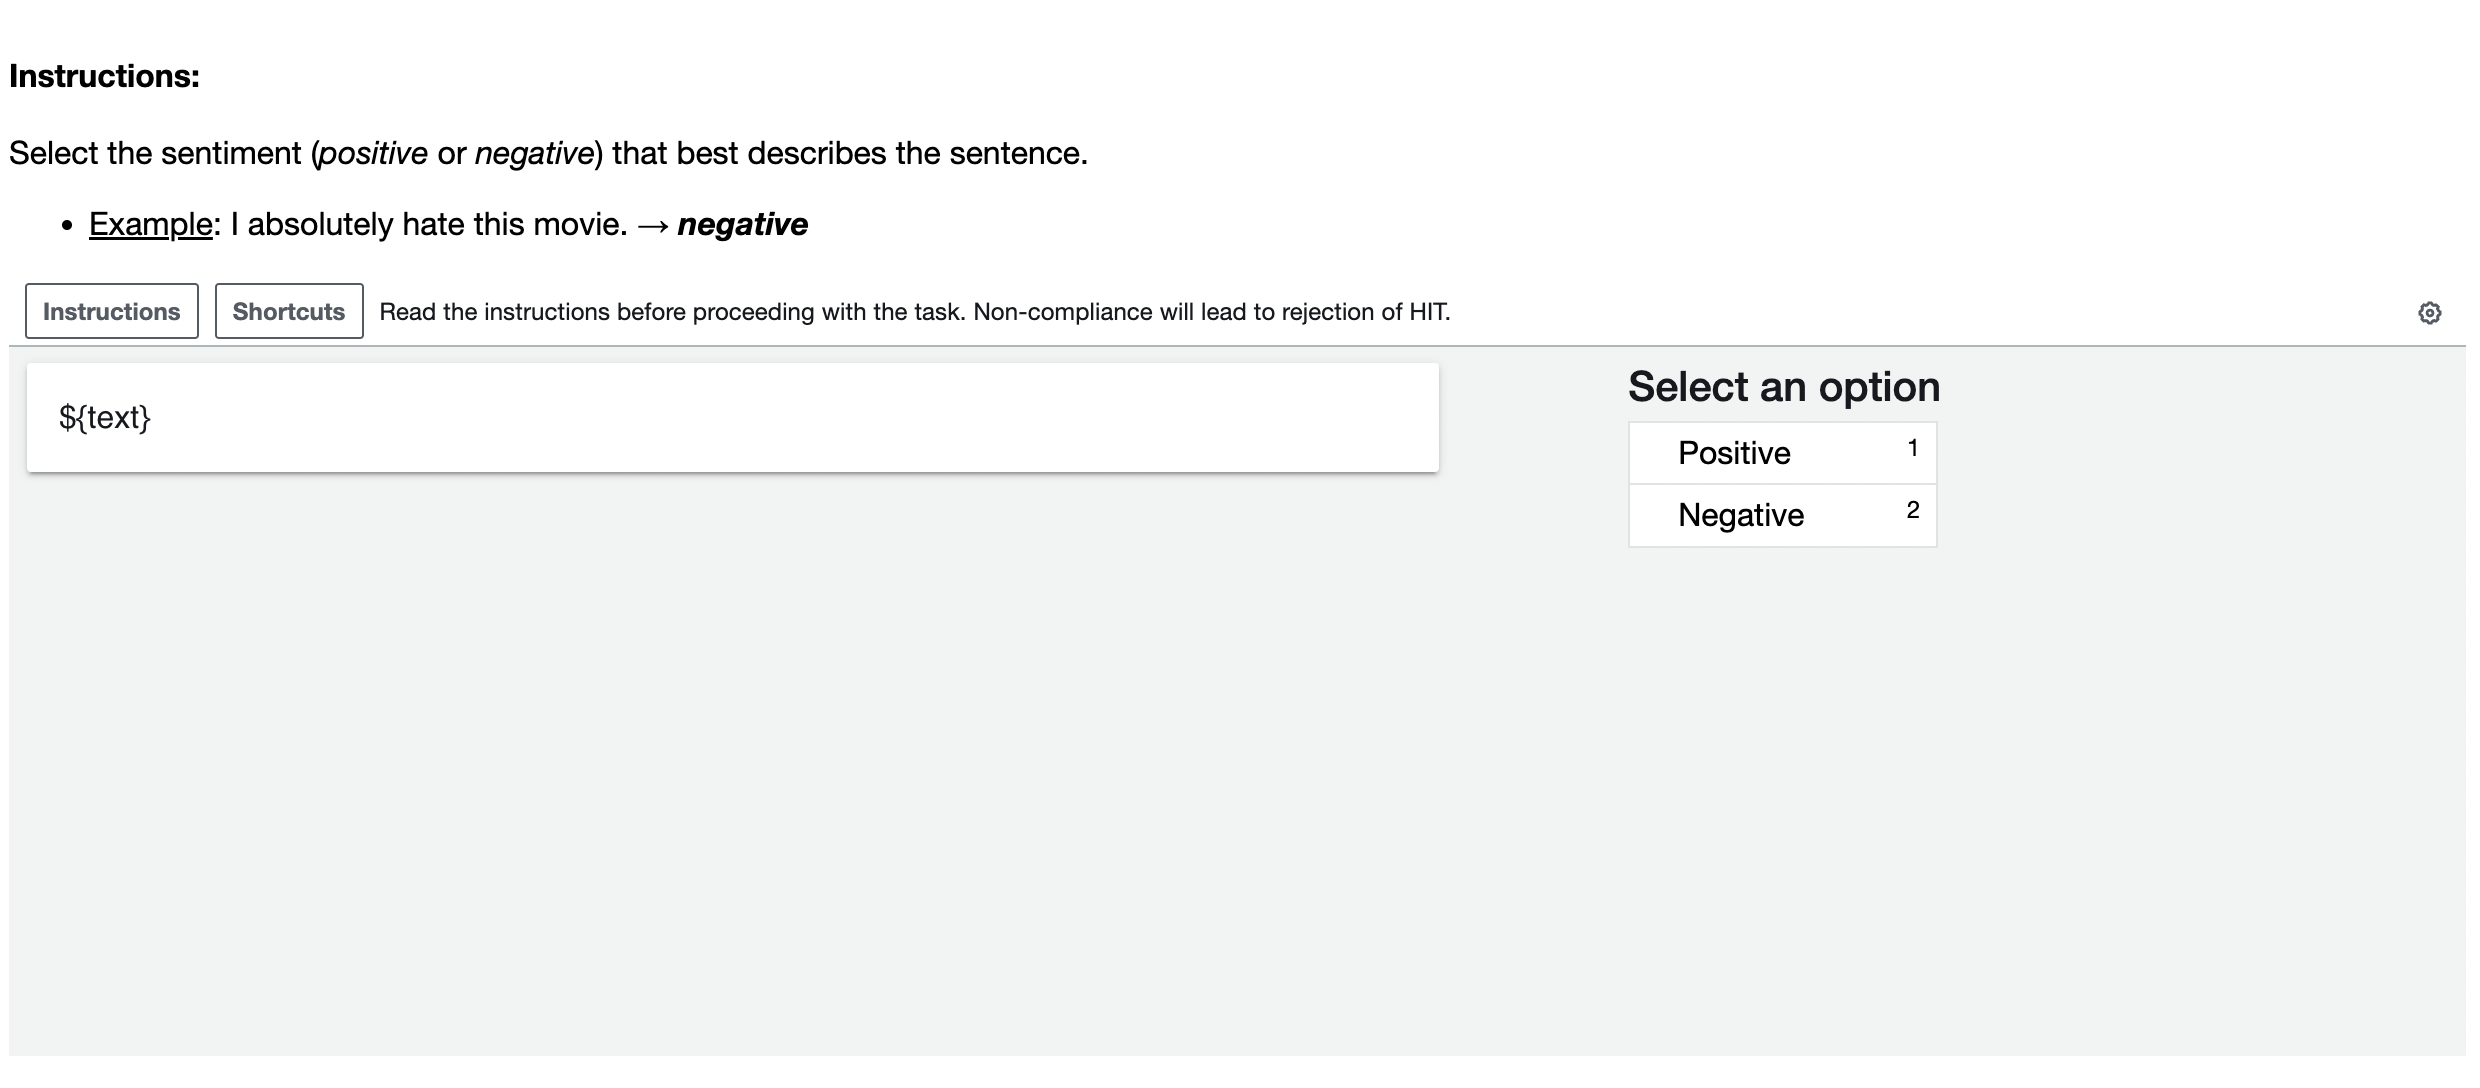}
    \caption{\textbf{Only Label:} Instructions and setup for Only Label annotation}
    \label{fig:app:rq4:task3}
\end{figure*}





\subsubsection{Task Setup}
Each task is timed and have the same set of $200$ instances to be annotated. Each instance is annotated by three annotators. 

Using the annotations we receive, we aggregate the time taken across all annotators and instances to obtain a rough time estimate taken to annotate \textit{one} instance for a given task.













































% Of the \aaron{XXXX} total dev instances, we see that there are \aaron{XXXX}, \aaron{XXXX}, \aaron{XXXX}, and \aaron{XXXX} instances in the $cor \hspace{-1mm} \rightarrow \hspace{-1mm} cor$, $incor \hspace{-1mm} \rightarrow \hspace{-1mm} incor$, $incor \hspace{-1mm} \rightarrow \hspace{-1mm} cor$, and $cor \hspace{-1mm} \rightarrow \hspace{-1mm} incor$ groups, respectively.

% \aaron{Summarize this better.}
% \aaron{Instead of this plot, make this table: (1) bin all points w.r.t. vanilla target class conf (can play around with number of bins); (2) for each bin, report the fraction of points in the incor --> cor group}

% These first two groups tend to  impacted by ER, as the model's predicted class is unchanged.


% Given that $\mathcal{F}$ achieves high ID task performance both with and without ER, we see that \aaron{XXXX} dev instances are in the $cor \hspace{-1mm} \rightarrow \hspace{-1mm} cor$ group, with high target class confidence with/without ER.
% Meanwhile, \aaron{XXXX} dev instances are in the $incor \hspace{-1mm} \rightarrow \hspace{-1mm} incor$ group, with low target class confidence with/without ER.

% On the other hand, there are \aaron{XXXX} and \aaron{XXXX} instances are in the $incor \hspace{-1mm} \rightarrow \hspace{-1mm} cor$ and $cor \hspace{-1mm} \rightarrow \hspace{-1mm} incor$ groups, respectively.
























% \begin{table}[]
% \begin{tabular}{cccccc}
% \toprule
% \textbf{ER criteria} & \textbf{\begin{tabular}[c]{@{}c@{}}V1: Sentiment-laden\\ words in Context\end{tabular}} & \textbf{\begin{tabular}[c]{@{}c@{}}V2: Changing\\ Neutral \\ Words\end{tabular}} & \textbf{\begin{tabular}[c]{@{}c@{}}N1: Adding \\ Simple \\ Negations\end{tabular}} & \textbf{\begin{tabular}[c]{@{}c@{}}N2: Addition\\ Simple \\ Non-Negations\end{tabular}} & \textbf{\begin{tabular}[c]{@{}c@{}}N3: Negation\\ interspersed \\ with Neutral Words\end{tabular}} \\
% \midrule
% \textbf{None} & 1.4 & 6.0 & 9.0 & 49.6 & 49.4 \\
% \textbf{MAE} & \textbf{0.4} & \textbf{5.0} & \textbf{2.6} & \textbf{35.2} & \textbf{21.0} \\
% \bottomrule
% \end{tabular}
% \end{table}
















% % \begin{table*}[t]
% \begin{table}[]
% % \vspace{-0.2cm}
% \centering
% \scalebox{0.6}{
% \begin{tabular}{cccccc}
%     \toprule
%     \multirow{4}{*}{\textbf{ER criteria}} & \multicolumn{4}{c}{\textbf{Sentiment Analysis}} \\
%     \cmidrule(lr){2-5}
%     & In-Domain & \multicolumn{3}{c}{Out-of-Domain} \\
%     \cmidrule(lr){2-2} \cmidrule(lr){3-5}
%     & SST & Amazon & Yelp & Movies \\
    
%     \midrule
    
%     {None} & 94.22~($\pm$0.77) & 90.72~($\pm$1.36) & 92.07~($\pm$2.66) & 89.83~($\pm$6.79) \\
    
%     \midrule
    
%     {MAE ($\lambda_{\text{ER}}=0.5$)} & \textbf{94.44~($\pm$0.24)} & 90.12~($\pm$2.98) & 92.27~($\pm$3.29) & 92.00~($\pm$5.68) \\
%     {MAE ($\lambda_{\text{ER}}=1$)} & 94.11~($\pm$0.38) & 92.02~($\pm$0.25) & 94.55~($\pm$0.30) & 95.50~($\pm$1.32) \\
%     {MAE ($\lambda_{\text{ER}}=10$)} & 94.26~($\pm$0.11) & 91.27~($\pm$0.28) & 93.10~($\pm$1.08) & 90.67~($\pm$3.79) \\
%     {MAE ($\lambda_{\text{ER}}=100$)} & 94.32~($\pm$0.13) & \textbf{92.33~($\pm$0.28)} & \textbf{94.92~($\pm$0.56)} & \textbf{95.50~($\pm$0.50)} \\
%     {MAE ($\lambda_{\text{ER}}=300$)} & 94.32~($\pm$0.05) & 91.83~($\pm$0.42) & 93.97~($\pm$1.28) & 95.00~($\pm$0.50) \\
    
%     \midrule
    
%     {MAE ($\gamma_{\text{ER}}=1$)} & \textbf{94.37~($\pm$0.11)} & 90.63~($\pm$1.88) & 92.32~($\pm$2.23) & 88.67~($\pm$4.25) \\
%     {MAE ($\gamma_{\text{ER}}=10$)} & 94.18~($\pm$0.16) & \textbf{92.30~($\pm$1.21)} & 93.01~($\pm$2.14) & \textbf{96.83~($\pm$1.04)} \\
%     {MAE ($\gamma_{\text{ER}}=100$)} & 94.11~($\pm$0.38) & 92.02~($\pm$0.25) & \textbf{94.55~($\pm$0.30)} & 95.50~($\pm$1.32) \\
%     {MAE ($\gamma_{\text{ER}}=1000$)} & 94.19~($\pm$0.24) & 90.47~($\pm$2.06) & 92.80~($\pm$2.90) & 92.67~($\pm$6.25) \\
    
%     \midrule
    
%     {MAE ($\text{lr}=2\mathrm{e}{-4}$)} & 83.63~($\pm$0.80) & 89.35~($\pm$2.85) & 91.23~($\pm$2.84) & 93.00~($\pm$2.65) \\
%     {MAE ($\text{lr}=2\mathrm{e}{-5}$)} & \textbf{94.11~($\pm$0.38)} & \textbf{92.02~($\pm$0.25)} & \textbf{94.55~($\pm$0.30)} & \textbf{95.50~($\pm$1.32)} \\
%     {MAE ($\text{lr}=2\mathrm{e}{-6}$)} & 91.35~($\pm$0.45) & 88.60~($\pm$1.60) & 83.27~($\pm$6.49) & 81.17~($\pm$6.93) \\
    
    
%     \bottomrule 
% \end{tabular}
% }
% % \vspace{0.3cm}
% \caption{\small \textbf{Task Performance \versus \{ER Strength ($\lambda_{\text{ER}}$), Rationale Scaling Factor ($\gamma_{\text{ER}}$)\}.} Higher values are better.}
% \label{tab:exp:use:hparam}
% % \vspace{-0.3cm}
% % \end{table*}
% \end{table}


% \subsubsection{ER Instance Prioritization}
% \label{sec:exp:use:instance}

% % \aaron{Update this.}
% % To further show the utility of \method, we pilot studies on ER instance prioritization in a human-in-the-loop learning setting.
% In \textsection \ref{sec:exp:ext}, we assumed that all instances in the training set have human rationale annotations.
% % $b_{\text{ER}} = |\mathcal{D}_{\text{train}}| k / 100$
% However, in real-world scenarios, we typically have a limited budget of human rationales.
% Given an annotation budget of $k\%$ of the training instances, how do we prioritize which $k\%$ to annotate for ER?
% In \textsection \ref{sec:exp:ext:conf}, we found that instances for which $\mathcal{F}_{\text{No-ER}}$ predicted low target class confidence tended to benefit most from ER.
% Thus, we propose to annotate the bottom-$k\%$ instances, w.r.t. $\mathcal{F}_{\text{No-ER}}$'s predicted target class confidence.
% We call this instance prioritization strategy Low-Conf.
% % We consider the event anchor detection task (a form of token classification), which ... \aaron{Explain what event anchor detection is}.
% % For event anchor detection, we consider an in-house dataset ... \aaron{Insert name of dataset}, which ... \aaron{Add details about event anchor detection dataset.} and crucially has no pre-annotated human rationales.
% % \aaron{Describe how rationales are annotated and why they are especially costly to annotate.}
% % Using $k=20$, we annotated the $k\%$ lowest-confidence train instances in the dataset.
% % As a baseline, we also separately annotated three uniform samples (without replacement) of $k\%$ instances.
% As a baseline strategy (Rand), we also annotate a random sample of $k\%$ instances.
% % Note that it is possible for the three random samples to overlap, in which case the overlapping instances were only annotated once.
% Note that Low-Conf and Rand instances may overlap, so overlapping instances are only annotated once.
% After that, we separately train $\mathcal{F}_{\text{ER}}$ using each set of human rationales, skipping ER for non-annotated instances.
% % (see \textsection \aaron{Add ref} for training details).
% % We report the random baseline task performance as the mean task performance across the three random samples.

% In Table \ref{tab:exp:use:instance}, we report ID/OOD task performance for both strategies on sentiment analysis and NER, using $k=15$ and the MAE ER criteria
% We also compare to the None baseline, which does not use ER or any human rationales.
% For ID (SST, CoNLL-2003), we find that None slightly beats both strategies.
% This is not surprising, as Table \ref{tab:exp:ext:task_perf} showed ER's limited improvement on ID task performance.
% However, for OOD (Amazon, Yelp, Movies, OntoNotes v5.0), the results are more interesting.
% For Amazon and OntoNotes v5.0, all three methods perform similarly.
% Meanwhile, for Yelp and especially Movies, Low-Conf outperforms None and Rand.
% This shows that target class confidence can be a predictive feature for ER instance prioritization, thus demonstrating \method's utility given limited rationale annotations.


% % In future work, we plan to explore more strategies for instance prioritization, beyond the lowest-confidence strategy used here.
% % We also plan to experiment with other tasks/datasets, besides event anchor detection and \aaron{Add dataset name}.
% % Also, the current rationale annotation scheme is relatively limited (\ie provide binary label for each token w.r.t. each class), so we plan to investigate more sophisticated techniques for annotating rationales.
% % In addition, the instance annotation budget does not need to be completely used in one annotation iteration. Instead, we could alternate between using a new part of the annotation budget and training $\mathcal{F}_{\text{task, ER}}$ with all rationales annotated so far.
% % That is, using a more updated version of $\mathcal{F}_{\text{task, ER}}$ to prioritize instances may yield better results.



% \subsection{Low-Resource Learning with \method}
% \subsubsection{ER Instance Prioritization}

% \begin{table*}[ht]
% % \vspace{-0.2cm}
% \centering
% \scalebox{0.68}{
% \begin{tabular}{ccccccc}
%     \toprule
%     \multirow{4}{*}{\textbf{ER criteria}} & \multicolumn{4}{c}{\textbf{Sentiment Analysis}} & \multicolumn{2}{c}{\textbf{NER}} \\
%     \cmidrule(lr){2-5} \cmidrule(lr){6-7}
%     & In-Domain & \multicolumn{3}{c}{Out-of-Domain} & In-Domain & \multicolumn{1}{c}{Out-of-Domain} \\
%     \cmidrule(lr){2-2} \cmidrule(lr){3-5} \cmidrule(lr){6-6} \cmidrule(lr){7-7}
%     & SST & Amazon & Yelp & Movies & CoNLL-2003 & OntoNotes v5.0 \\
    
%     \midrule
    
%     % {None} & 94.22~($\pm$0.77) & 90.72~($\pm$1.36) & 92.07~($\pm$2.66) & 89.83~($\pm$6.79) & 77.24~($\pm$0.20) & 20.78~($\pm$0.41) \\
    
%     % \midrule
    
%     % {None} & 94.22~($\pm$0.77) & 90.72~($\pm$1.36) & 92.07~($\pm$2.66) & 89.83~($\pm$6.79) & \textbf{77.24~($\pm$0.20)} & 20.78~($\pm$0.41) \\
     
%     % {MAE (5$\%$ Rand)} & 94.06~($\pm$0.64) & \textbf{91.51~($\pm$1.03)} & 92.34~($\pm$3.89) & \textbf{92.11~($\pm$6.07)} & 75.35~($\pm$1.48) & \textbf{20.83~($\pm$0.48)} \\
    
%     % {MAE (5$\%$ Low-Conf)} & \textbf{94.25~($\pm$0.28)} & 90.58~($\pm$0.83) & \textbf{92.53~($\pm$0.42)} & 86.83~($\pm$7.01) & 75.44~($\pm$1.07) & 20.27~($\pm$0.35) \\
    
%     % \midrule
    
%     % {None} & 94.22~($\pm$0.77) & 90.72~($\pm$1.36) & 92.07~($\pm$2.66) & 89.83~($\pm$6.79) & \textbf{77.24~($\pm$0.20)} & 20.78~($\pm$0.41) \\
    
%     % {MAE (10$\%$ Rand)} & 94.25~($\pm$0.29) & \textbf{91.28~($\pm$0.85)} & \textbf{93.63~($\pm$1.09)} & \textbf{95.22~($\pm$1.77)} & 75.76~($\pm$0.82) & \textbf{20.86~($\pm$0.24)} \\
    
%     % {MAE (10$\%$ Low-Conf)} & \textbf{94.31~($\pm$0.88)} & 91.05~($\pm$1.39) & 93.58~($\pm$1.78) & 94.00~($\pm$0.87) & 75.84~($\pm$0.94) & 20.50~($\pm$0.24) \\
    
%     % \midrule
    
%     {None} & \textbf{94.22~($\pm$0.77)} & 90.72~($\pm$1.36) & 92.07~($\pm$2.66) & 89.83~($\pm$6.79) & \textbf{77.24~($\pm$0.20)} & 20.78~($\pm$0.41) \\
    
%     {MAE (15$\%$ Rand)} & 93.37~($\pm$0.85) & \textbf{91.18~($\pm$1.12)} & 93.05~($\pm$1.76) & 92.83~($\pm$4.37) & 76.90~($\pm$0.65) & \textbf{20.97~($\pm$0.55)} \\
    
%     {MAE (15$\%$ Low-Conf)} & 94.20~($\pm$0.56) & 90.89~($\pm$1.60) & \textbf{94.07~($\pm$0.84)} & \textbf{95.33~($\pm$0.58)} & 74.99~($\pm$1.00) & 20.53~($\pm$0.25) \\
    
%     \bottomrule 
% \end{tabular}
% }
% % \vspace{0.3cm}
% \caption{\small \textbf{Instance Prioritization.} Higher values are better.}
% \label{tab:exp:use:instance}
% % \vspace{-0.3cm}
% \end{table*}












% \begin{table*}[ht]
% % \centering
% \begin{center}
% \scalebox{0.60}{
% \begin{tabular}{ccccccccccccc}
%     \toprule
%     \multirow{2}{*}{\textbf{ER criteria}} & \multicolumn{10}{c}{\textbf{Stress Test}} \\
%     \cmidrule(lr){2-11}
%     & \multicolumn{5}{c}{\textbf{Sentiment Analysis}} & \multicolumn{5}{c}{\textbf{NLI}}\\
%     \cmidrule(lr){2-6} \cmidrule(lr){7-11}
%     & Vocab. & Robust. & Logic & Entity. & Overall & Vocab. & Robust. & Logic & Entity. & Overall\\
%     \midrule
%     {None} & 9.51~($\pm$2.9) & 4.25~($\pm$0.58) & 32.38~($\pm$8.96) & 1.61~($\pm$0.29) &  10.6~($\pm$2.83) & 42.9~($\pm$14.78) & 17.61~($\pm$4.56) & 54.99~($\pm$13.73) & \textbf{77.21~($\pm$39.57)} & 40.12~($\pm$13.03)\\
%     \midrule
%     {MSE}  & 9.94~($\pm$8.41) & \textbf{3.28~($\pm$1.01)} & 32.8~($\pm$6.46) & 1.72~($\pm$0.73) &  10.57~($\pm$4.53) & \textbf{33.29~($\pm$11.07)} & 13.53~($\pm$4.09) & \textbf{46.88~($\pm$17.05)} & 88.88~($\pm$24.11) & 34.87~($\pm$11.35)\\
%     {MAE}  & 9.47~($\pm$1.97) & 3.96~($\pm$0.83) & \textbf{25.65~($\pm$10)} & 1.66~($\pm$0.59) &  9.32~($\pm$2.81) & 42.81~($\pm$8.22) & 15.4~($\pm$3.52) & 40.3~($\pm$16.05) & 79.91~($\pm$22.2) & 35.53~($\pm$9.92)\\
%     {BCE}  & 8.84~($\pm$5.33) & 3.76~($\pm$1.1) & 28.91~($\pm$9.34) & \textbf{1.49~($\pm$0.75)} &  9.59~($\pm$3.98) & 33.7~($\pm$11.39) & 12.36~($\pm$3.67) & 52.71~($\pm$18.93) & 85.18~($\pm$30.04) & 35.8~($\pm$12.33)\\
%     {Huber} & 8.32~($\pm$3.49) & 4.35~($\pm$0.49) & 34.64~($\pm$6.95) & 1.74~($\pm$0.46) &  10.64~($\pm$2.68) & 38.1~($\pm$11.85) & 14.48~($\pm$3.91) & 42.67~($\pm$14.15) & 83.83~($\pm$24.25) & 34.92~($\pm$10.72)\\
%     {Order} & \textbf{4.63~($\pm$1.07)} & 3.63~($\pm$0.88) & 26.89~($\pm$12.14) & 1.93~($\pm$1.3) &  \textbf{7.79~($\pm$3.01)} & 35.12~($\pm$9.07) & \textbf{11.37~($\pm$3.23)} & 45.23~($\pm$11.23) & 96.4~($\pm$4.85) & \textbf{34.81~($\pm$7.15)}\\
    
%     \bottomrule 
% \end{tabular}
% }
% % \vspace{0.3cm}
% \caption{\small \textbf{Stress Tests.}}
% \label{tab:exp:ext:stress_test}
% % \vspace{-0.3cm}
% \end{center}
% \end{table*}





  
    






























% \begin{table*}[t]
% % \vspace{-0.2cm}
% \centering
% \scalebox{0.7}{
% \begin{tabular}{ccccccccc}
%     \toprule
%     \multirow{4}{*}{\textbf{ER criteria}} & \multicolumn{4}{c}{\textbf{Sentiment Analysis}} & \multicolumn{2}{c}{\textbf{NER}} \\
%     \cmidrule(lr){2-5} \cmidrule(lr){6-7}
%     & In-Domain & \multicolumn{3}{c}{Out-of-Domain} & In-Domain & \multicolumn{1}{c}{Out-of-Domain} \\
%     \cmidrule(lr){2-2} \cmidrule(lr){3-5} \cmidrule(lr){6-6} \cmidrule(lr){7-7}
%     & SST & Amazon & Yelp & Movies & CoNLL03 & OntoNotes \\
%     \midrule
%     {None} & 0.00~($\pm$0.00) & 0.00~($\pm$0.00) & 0.00~($\pm$0.00) & 0.00~($\pm$0.00) & 0.00~($\pm$0.00) & 0.00~($\pm$0.00) \\
%     \midrule
%     {MSE} & 0.32~($\pm$1.05) & \textbf{-1.25~($\pm$1.20)} &\textbf{-2.33~($\pm$4.64)} & -6.50~($\pm$40.66) & X.XX~($\pm$X.XX) & X.XX~($\pm$X.XX) \\
%     {MAE} & -0.09~($\pm$0.24) & -0.58~($\pm$3.45) & -0.94~($\pm$11.21) & \textbf{-7.00~($\pm$40.66)} & X.XX~($\pm$X.XX) & X.XX~($\pm$X.XX) \\
%     {BCE} & \textbf{-0.16~($\pm$0.33)} & 0.46~($\pm$4.11) & 0.96~($\pm$26.99) & 0.16~($\pm$47.72) & X.XX~($\pm$X.XX) & X.XX~($\pm$X.XX) \\
%     {Huber} & 0.12~($\pm$0.42) & 0.19~($\pm$2.25) & -1.05~($\pm$4.11) & -4.33~($\pm$37.72) & X.XX~($\pm$X.XX) & X.XX~($\pm$X.XX) \\
%     {Order} & 1.90~($\pm$1.38) & 6.98~($\pm$3.87) & 19.86~($\pm$45.54) & 21.66~($\pm$35.72) & X.XX~($\pm$X.XX) & X.XX~($\pm$X.XX) \\
    
%     \bottomrule 
% \end{tabular}
% }
% % \vspace{0.3cm}
% \caption{\small \textbf{ID/OOD Opportunity Cost.} Lower values are better.}
% \label{tab:opp_cost}
% % \vspace{-0.3cm}
% \end{table*}






% \begin{table*}[t]
% % \vspace{-0.2cm}
% \centering
% \scalebox{0.7}{
% \begin{tabular}{ccccccccc}
%     \toprule
%     \multirow{4}{*}{\textbf{ER criteria}} & \multicolumn{4}{c}{\textbf{Sentiment Analysis}} & \multicolumn{2}{c}{\textbf{NER}} \\
%     \cmidrule(lr){2-5} \cmidrule(lr){6-7}
%     & In-Domain & \multicolumn{3}{c}{Out-of-Domain} & In-Domain & \multicolumn{1}{c}{Out-of-Domain} \\
%     \cmidrule(lr){2-2} \cmidrule(lr){3-5} \cmidrule(lr){6-6} \cmidrule(lr){7-7}
%     & SST & Amazon & Yelp & Movies & CoNLL03 & OntoNotes \\
%     \midrule
%     {None} & 94.22~($\pm$0.77) & 90.72 ($\pm$1.36) & 92.07~($\pm$2.66) & 89.83~($\pm$6.79) & 75.73~($\pm$0.61) & 21.36~($\pm$0.38) \\
%     \midrule
%     {MSE} & 94.14~($\pm$0.19) & \textbf{91.98~($\pm$0.38)} & \textbf{94.40~($\pm$0.33)} & 96.33~($\pm$1.26) & 75.15~($\pm$0.77) & 21.84~($\pm$0.86) \\
%     {MAE} & 94.18~($\pm$0.16) & 91.30~($\pm$1.21) & 93.02~($\pm$2.14) & \textbf{96.83~($\pm$1.04)} & \textbf{76.25~($\pm$1.55)} & \textbf{22.08~($\pm$0.12)} \\
%     {BCE} & 94.19~($\pm$0.19) & 90.25~($\pm$1.65) & 91.12~($\pm$4.56) & 89.67~($\pm$5.53) & 75.45~($\pm$0.91) & 21.50~($\pm$0.63) \\
%     {Huber} & 94.21~($\pm$0.11) & 90.52~($\pm$0.71) & 93.12~($\pm$0.29) & 83.83~($\pm$17.19) & 74.51~($\pm$1.13) & 21.19~($\pm$0.16) \\
%     {Order} & \textbf{94.35~($\pm$0.08)} & 83.77~($\pm$3.46) & 72.22~($\pm$10.13) & 78.67~($\pm$14.94) & 75.69~($\pm$0.58) & 21.39~($\pm$0.86) \\
    
%     \bottomrule 
% \end{tabular}
% }
% % \vspace{0.3cm}
% \caption{\small \textbf{ID/OOD Task Performance.} Higher values are better. \aaron{Using rationale scaling factor 1?}}
% \label{tab:task_perf_old}
% % \vspace{-0.3cm}
% \end{table*}

% TBD

% \begin{table*}[ht]
% % \vspace{-0.2cm}
% \centering
% \scalebox{0.48}{
% \begin{tabular}{cccccccccccc}
%     \toprule
%     \multirow{4}{*}{\textbf{ER Criteria}} & \multicolumn{4}{c}{\textbf{Sentiment Analysis}} & \multicolumn{2}{c}{\textbf{NLI}} & \multicolumn{2}{c}{\textbf{NER}} & \multicolumn{3}{c}{\textbf{Hate Speech Detection}} \\
%     \cmidrule(lr){2-5} \cmidrule(lr){6-7} \cmidrule(lr){8-9} \cmidrule(lr){10-12}
%     & In-Distribution & \multicolumn{3}{c}{Out-of-Distribution} & In-Distribution & \multicolumn{1}{c}{Out-of-Distribution} & In-Distribution & \multicolumn{1}{c}{Out-of-Distribution} & In-Distribution & \multicolumn{2}{c}{Out-of-Distribution} \\
%     \cmidrule(lr){2-2} \cmidrule(lr){3-5} \cmidrule(lr){6-6} \cmidrule(lr){7-7} \cmidrule(lr){8-8} \cmidrule(lr){9-9} \cmidrule(lr){10-10} \cmidrule(lr){11-12}
%     & SST & Amazon & Yelp & Movies & e-SNLI & MNLI & CoNLL-2003 & OntoNotes v5.0 & Stf. & HatEval & GHC\\
%     \midrule
%     {None} & 94.22~($\pm$0.77) & 90.72 ($\pm$1.36) & 92.07~($\pm$2.66) & 89.83~($\pm$6.79) & 76.18~($\pm$1.28) & 46.15~($\pm$4.38) & 77.24~($\pm$0.20) & 20.78~($\pm$0.41) & 89.50~($\pm$0.20) & 63.68~($\pm$0.78) & 89.43~($\pm$0.98) \\
%     \midrule
%     {MSE}  & 94.29~($\pm$0.05) & 90.58~($\pm$0.77) & 92.17~($\pm$0.64) & 90.00~($\pm$5.63) & 78.98~($\pm$1.00) & 54.23~($\pm$2.67) & 78.02~($\pm$0.69) & 21.60~($\pm$0.46) & 89.46~($\pm$0.21) & 64.30~($\pm$1.52) & 89.43~($\pm$0.98)\\
%     {MAE}  & 94.11~($\pm$0.38) & \textbf{92.02~($\pm$0.25)} & \textbf{94.55~($\pm$0.30)} & \textbf{95.50~($\pm$1.32)} & 78.77~($\pm$1.01) & 52.41~($\pm$4.50) & \textbf{78.34~($\pm$0.81)} & \textbf{21.73~($\pm$0.31)} & \textbf{89.59~($\pm$0.06)} & 63.30~($\pm$0.49) & 88.07~($\pm$1.66)\\
%     {BCE} & 94.15~($\pm$0.53) & 90.70~($\pm$1.19) & 91.82~($\pm$2.30) & 92.00~($\pm$6.98) & 79.07~($\pm$0.83) & 53.68~($\pm$4.15) & 64.53~($\pm$13.22) & 17.32~($\pm$3.59) & 89.42~($\pm$0.71) & 63.54~($\pm$0.57) & 88.99~($\pm$0.83)\\
%     {Huber} & 94.19~($\pm$0.19) & 90.43 ($\pm$1.45) & 92.38~($\pm$2.11) & 91.83~($\pm$3.75) & 78.99~($\pm$0.81) & 53.97~($\pm$3.11)& 77.83~($\pm$1.09) & 21.38~($\pm$0.16)& 89.50~($\pm$0.51) & \textbf{64.85~($\pm$1.50)} & 87.77~($\pm$1.21) \\
%     {Order} & \textbf{94.37~($\pm$0.11)} & 89.47 ($\pm$2.71) & 87.95~($\pm$6.36) & 84.50~($\pm$10.15) & \textbf{79.11~($\pm$0.87)} & \textbf{55.26~($\pm$3.56)}  & 72.62~($\pm$5.01) & 19.14~($\pm$1.75)& 89.21~($\pm$1.18) & 64.46~($\pm$1.18) & \textbf{92.84~($\pm$0.46)} \\
    
%     \bottomrule 
% \end{tabular}
% }
% % \vspace{0.3cm}
% \caption{\small \textbf{ID/OOD Task Performance (Instance-Based Human Rationales).} This table enlists the ID and OOD performance of different ER criteriona (MSE, MAE, BCE, Huber, Order) and compares them to a setting without ER (None). All models (with or without ER) are trained on the ID dataset and evaluated on the ID and OOD datasets without the need of machine or human rationales. Metrics displayed here (higher the better) for sentiment analysis is Accuracy and Macro F1 for NLI and NER.}
% \label{tab:exp:rq1:unseen}
% % \vspace{-0.3cm}
% \end{table*}
